# Supplementary material for: Improving Implicit Regularization of SGD with Preconditioning for Least Square Problems
Source: arXiv:2403.08585 source file (2024-05-26)
Supplement: Supplementary file 1 [file precond_sgd_outperformance_standard_ridge.tex]

\newpage
\section{Analysis of precondition SGD with standard ridge regression}
\begin{theorem}[preconditioned SGD outperformance ridge]\label{thm:H_I}
Let
$$\Gb = \big ( \beta \Hb + \Ib \big )^{-1},$$
and 
$$\beta = \frac{N}{\log N \tr(\Hb)}$$

Let $\wb_{\mathrm{sgd}}(N; \Gb, \gamma)$ and $\wb_{\mathrm{ridge}}(N; \lambda)$ be the solutions found by the pre-conditioned SGD and ridge regression respectively. Then under Assumption~\ref{assump:fourth_moment},~\ref{assump:model_noise}, for any least square problem instance such that the ridge regression solution is generalizable  and any $\lambda$, there exists a choice of stepsize $\gamma^*$ for preconditioned-SGD such that

\begin{align*}
L\big[\wb_{\mathrm{sgd}}(N, \Gb; \gamma^*)\big]-L(\wb^*)\lesssim L\big[\wb_{\mathrm{ridge}}(N;\lambda)\big] -L(\wb^*),
\end{align*}
\end{theorem}

\begin{lemma}\label{lemma:tilde_eigen}
    Suppose $$\Gb = \big ( \beta \Hb + \Ib \big )^{-1}, \quad \tilde{\Hb} = \Gb^{1/2} \Hb \Gb^{1/2} $$
    then we have 
    $$\tilde{\lambda}_i = \frac{\lambda_i}{\beta \lambda_i + 1}.$$
\end{lemma}
\begin{proof}
    Let $\vb_i$ be an arbitrary eigenvector of $\Hb$ with eigenvalue $\lambda_i \geq 0$. Then, it is an eigenvector for $\beta \Hb + \Ib$ with eigenvalue $\beta \lambda_i + 1 > 0$. 
    Therefore, it is also an eigenvector for $\Gb = (\beta \Hb + \Ib)^{-1}$ with eigenvalue $\frac{1}{\beta \Hb + \Ib}$. 

    Since $\Gb$ is PSD matrix, $\Gb^{1/2}$ and $\Gb$ have the same eigenvectors. Therefore we have that $\Gb^{1/2}\Hb\Gb^{1/2}$, $\Gb\Hb$ and $\Hb$ have the same eigenvectors. Furthermore, we have that the $i$-th eigenvalues of  $\Gb^{1/2}\Hb\Gb^{1/2} $ is 
    $$\Gb^{1/2}\Hb\Gb^{1/2} = \Gb\Hb[i] = \frac{\lambda_i}{\beta \lambda_i + 1} $$
\end{proof}

\begin{lemma}\label{lemma:trace_rel}
    $\tr(\tilde{\Hb}) \leq \tr({\Hb})$
\end{lemma}
\begin{proof}
    By the choice of $\beta$, we have that 
    $$\beta \lambda_i + 1 \geq 1.$$
    Therefore, we have
    $$\tilde{\lambda}_i \leq \lambda_i$$
    This leads to 
    $$\tr(\tilde{\Hb}) = \sum_{i} \tilde{\lambda}_i \leq \sum_{i} {\lambda}_i = \tr(\Hb)$$
\end{proof}

\begin{lemma}\label{lemma:monotone}
    For $i \in [d-1]$, we have $$\tilde{\lambda}_{i+1} \leq \tilde{\lambda}_{i}.$$
\end{lemma}
\begin{proof}
    Let's denote $\tilde{\lambda} = f(\lambda) = \frac{\lambda}{\beta \lambda + 1}$. By taking the derivative of $f(\lambda)$ with respect to $\lambda$, we get that 
    \begin{align*}
        \frac{\partial f(\lambda)}{\partial \lambda} &= \frac{\beta \lambda + 1 - \beta \lambda}{(\beta \lambda +1)^2}\\
        &= \frac{1}{(\beta \lambda +1)^2} \\
        &> 0
    \end{align*}
    Therefore, $f(\lambda)$ is an increasing function with respect to $\lambda$. 
    By set up, we have that $\lambda_{i+1} \leq \lambda_{i}$. Combining the monotonicity of $f(\lambda)$, we have that
    $$f(\lambda_{i+1}) \leq  f(\lambda_{i}) \implies \tilde{\lambda}_{i+1} \leq \tilde{\lambda}_i $$
\end{proof}

\begin{proof}[Proof of Theorem~\ref{thm:H_I}]
By Theorem~\ref{theorem:precondition_sgd_fit2}, the learning dynamic of SGD after preconditioning can be characterized by $\tilde{\Hb} = \Gb^{1/2}\Hb\Gb^{1/2}$. By Lemma~\ref{lemma:tilde_eigen}, we can obtain the following eigenspectrum of $\tilde{\Hb}$:
$$\tilde{\lambda}_i = \frac{\lambda_i}{\beta \lambda_i + 1}.$$
Again, by Theorem~\ref{theorem:precondition_sgd_fit2}, we know the the excessive risk of preconditioned SGD is given by the following, where the parameter $k_1,k_2\in[d]$ can be arbitrarily chosen:
\begin{equation}
    \begin{split}
        \mathrm{SGDRiskBound}
&\lesssim \underbrace{\frac{1}{\eta^2 N^2}\cdot\big\|\exp(-N\eta \tilde{\Hb})\tilde{\wb}^*\big\|_{\tilde{\Hb}_{0:k_1}^{-1}}^2 + \|\tilde{\wb}^*\big\|_{\tilde{\Hb}_{k_1:\infty}}^2}_{\mathrm{SGDBiasBound}} \\
&\qquad + \underbrace{\bigg (\sigma^2+\frac{\|\tilde{\wb}^*\|^2_{\Ib_{0:k_2}}+N\eta \|\tilde{\wb}^*\|^2_{\tilde{\Hb}_{k_2:\infty}} }{N\eta} \bigg)\cdot\bigg(\frac{k_2}{N}+N\eta^2\sum_{i>k_2}\tilde{\lambda}_i^2\bigg)}_{\mathrm{SGDVarianceBound}}.
    \end{split}
\end{equation}

Then recall the lower bound of the risk achieved by ridge regression with parameter $\lambda$:
\begin{equation}
    \begin{split}
        \mathrm{RidgeRiskBound}
\gtrsim \underbrace{\frac{\hat{\lambda}^2}{ N^2}\cdot\big\|\wb^*\big\|_{\Hb_{0:k^*}^{-1}}^2 + \|\wb^*\big\|_{\Hb_{k^*:\infty}}^2}_{\mathrm{RidgeBiasBound}} 
 + \underbrace{\sigma^2\cdot\bigg(\frac{k^*}{N}+\frac{N}{\hat{\lambda}^2}\sum_{i>k^*}\lambda_i^2\bigg)}_{\mathrm{RidgeVarianceBound}},
    \end{split}
\end{equation}
where $\hat{\lambda} = \lambda + \sum_{i>k^*}\lambda_i$ and $k^* = \min \{k: \lambda_k \leq \frac{\lambda + \sum_{i>k}\lambda_i}{N}\}$. 

Then, we divide the analysis into two cases: {\bf Case I:} $\hat{\lambda} \geq \tr(\tilde{\Hb})$ and {\bf Case II:} $\hat{\lambda} < \tr(\tilde{\Hb})$.

For {\bf Case I}, we have that $\frac{1}{\hat{\lambda}} \leq \frac{1}{\tr(\tilde{\Hb})}$. We can set $\eta = \frac{1}{\hat{\lambda}}$ and $k_1,k_2 = k^*$. We divide the analysis into bias and variance. For the bias, we have that,

\begin{align*}
        \mathrm{SGDBiasBound}
& \lesssim \frac{\tilde{\lambda}^2}{ N^2}\cdot\bigg\|\exp(-\frac{N\tilde{\Hb}}{\tilde{\lambda}})\tilde{\wb}^*\bigg\|_{\tilde{\Hb}_{0:k^*}^{-1}}^2 + \|\tilde{\wb}^*\big\|_{\tilde{\Hb}_{k^*:\infty}}^2 \\
& \lesssim \frac{\tilde{\lambda}^2}{ N^2}\cdot\bigg\|\exp(-\frac{N\tilde{\Hb}}{\tilde{\lambda}}) \bigg \|^2 \big \| \tilde{\wb}^*\big\|_{{\Hb}_{0:k^*}^{-1}}^2 +  \|\tilde{\wb}^*\big\|_{\tilde{\Hb}_{k^*:\infty}}^2\\
 \shortintertext{By Lemma~\ref{lemma:double_effect}, we can obtain that,} 
& \lesssim \frac{\tilde{\lambda}^2}{ N^2}\cdot\bigg\|\exp(-\frac{N\tilde{\Hb}}{\tilde{\lambda}}) \bigg \|^2 \big \| {\wb}^*\big\|_{{\Hb}_{0:k^*}^{-1}}^2 + \|{\wb}^*\big\|_{{\Hb}_{k^*:\infty}}^2 \\
& \lesssim \frac{\tilde{\lambda}^2}{ N^2}\cdot \big \| {\wb}^*\big\|_{{\Hb}_{0:k^*}^{-1}}^2 + \|{\wb}^*\big\|_{{\Hb}_{k^*:\infty}}^2 \\
& \eqsim \mathrm{RidgeBiasBound}
\end{align*}

For the variance we have, 

\begin{align*}
        \mathrm{SGDVarianceBound}
& \lesssim \bigg (\sigma^2+\frac{\|\tilde{\wb}^*\|^2_{\Ib_{0:k^*}}+N\eta \|\tilde{\wb}^*\|^2_{\tilde{\Hb}_{k^*:\infty}} }{N\eta}\bigg)\cdot\bigg(\frac{k^*}{N}+N\eta^2\sum_{i>k^*}\tilde{\lambda}_i^2\bigg) \\
    \shortintertext{using the fact that $\beta \lambda_i + 1 \geq 1$, we have} 
 & \lesssim \bigg(1+\frac{\|\tilde{\wb}^*\|^2_{\Ib_{0:k^*}}+N\eta \|\tilde{\wb}^*\|^2_{\tilde{\Hb}_{k^*:\infty}} }{N\eta \sigma^2}\bigg)\cdot \sigma^2 \bigg(\frac{k^*}{N}+\frac{N}{\tilde{\lambda}^2}\sum_{i>k^*}{\lambda}_i^2\bigg)\\
&= \bigg(1+\frac{\|\tilde{\wb}^*\|^2_{\Ib_{0:k^*}}+N\eta \|\tilde{\wb}^*\|^2_{\tilde{\Hb}_{k^*:\infty}} }{N\eta \sigma^2}\bigg)\cdot \mathrm{RidgeVarianceBound}\\
& \lesssim \mathrm{RidgeVarianceBound}
\end{align*}

The last inequality is due to the assumption that we are in the generalizable region where the signal-to-noise ratio is reasonable and bounded.

Combining the result for both bias and variance, we have that 
$$ \mathrm{SGDRisk} \lesssim \mathrm{RidgeRisk}.$$

For {\bf Case II}, $\frac{1}{\hat{\lambda}} > \frac{1}{\tr(\tilde{\Hb})}$.  $\frac{1}{\hat{\lambda}}$ is no longer a feasible learning rate. By Lemma~\ref{lemma:trace_rel}, we can obtain that $\frac{1}{\tr(\Hb)}$ is a feasible learning rate. Therefore, we can set $\eta = \frac{1}{\tr (\Hb)}$ and $k_1,k_2 = k^*$. Similarly, we divide the analysis into bias and variance.

{\bf Bias.} The bias bound of preconditioned SGD is given as follows,

\begin{align*}
    \mathrm{SGDBiasBound}
&\lesssim \frac{1}{\eta^2 N^2}\cdot\big\|\exp(-N\eta \tilde{\Hb})\tilde{\wb}^*\big\|_{\tilde{\Hb}_{0:k^*}^{-1}}^2 + \|\tilde{\wb}^*\big\|_{\tilde{\Hb}_{k^*:\infty}}^2 \\
\end{align*}

For the bias, we can decompose the bias of SGD into two intervals: 1) $i \leq k^*$ and 2) $i > k^*$.

We start with the second interval. For $i > k^*$, by Lemma~\ref{lemma:double_effect}, we have that,
\begin{align*}
        \mathrm{SGDBiasBound}[i:\infty] & = \|\tilde{\wb}^*\big\|_{\tilde{\Hb}_{k^*:\infty}}^2 \notag \\
        & = \|\wb^*\big\|_{\Hb_{k^*:\infty}}^2 \\
        & = \mathrm{RidgeBiasBound}[i:\infty].
\end{align*}

For $i \leq k^*$, note that we can decompose each term of bias bound as follows, \dz{the notation $\hat \lambda$ and $\tilde \lambda$ look confusing.} \jw{I use $\hat{\lambda}$ to denote anything related to ridge and $\tilde{\lambda}$ to denote any thing related to sgd. I fixed some previous errors.}
\begin{align}
    \mathrm{SGDBiasBound[i]} &= (\tilde{\wb}^*[i])^2\frac{1}{N^2 \eta ^2\tilde{\lambda}_i}\exp \bigg(-2\eta N\tilde{\lambda}_i\bigg)  \notag\\
     &= (\wb^*[i])^2\frac{1}{N^2}\frac{1}{\lambda_i} \bigg (\frac{\beta\lambda_i + 1}{\eta} \bigg )^2\exp \bigg(-2\eta N\tilde{\lambda}_i\bigg)  \notag\\
     &= (\wb^*[i])^2\frac{1}{N^2}\frac{1}{\lambda_i} \hat{\lambda}^2 \frac{1}{\hat{\lambda}^2} \bigg (\frac{\beta\lambda_i + 1}{\eta} \bigg )^2\exp \bigg(-2\eta N\tilde{\lambda}_i\bigg)  \notag\\
     &= \mathrm{RidgeBiasBound}[i]  \bigg (\frac{\beta\lambda_i + 1}{\eta \hat{\lambda}} \exp \bigg(-\eta N\tilde{\lambda}_i\bigg)\bigg )^2  \label{eq:ridge_factor} \\
     \shortintertext{subsitute $\eta$, $\tilde{\lambda}_i$ and $\beta$ in (\ref{eq:ridge_factor}), we get:} 
     & =  \mathrm{RidgeBiasBound}[i]  \bigg ( \frac{\left( \lambda_i N/ (\log N \tr(\Hb)) + 1 \right)  \tr(\Hb)}{\hat{\lambda}} \exp \bigg(-\frac{1}{\tr(\Hb)} N \frac{\lambda_i}{\beta\lambda_i+1}\bigg)\bigg )^2 \label{eq:sgd_bias2}  
\end{align}

By Lemma~\ref{lemma:monotone}, we know that $\frac{\lambda_i}{\beta\lambda_i+1}$ is a monotonic increasing function. Therefore, we can obtain that,
\begin{align}
    \frac{\lambda_i}{\beta\lambda_i+1} \geq \frac{\lambda_{k^*}}{\beta \lambda_{k^*}+1}, \forall i \leq k^* \label{eq:tidle_lambda_lower}
\end{align}
Substitute the above fact (\ref{eq:tidle_lambda_lower}) into (\ref{eq:sgd_bias2}), we can obtain
\begin{align}
      \mathrm{SGDBiasBound[i]}  & \leq  \mathrm{RidgeBiasBound}[i] \left( \left( \frac{\lambda_i N }{\log N\hat{\lambda}} + \frac{\tr(\Hb)}{\hat{\lambda}}\right) \exp \bigg(-\frac{1}{\tr(\Hb)} N \frac{\lambda_{k^*}}{\beta\lambda_{k^*}+1}\bigg) \right)^2   \notag \\
      &\lesssim  \mathrm{RidgeBiasBound}[i] \left( \left( \frac{\lambda_i N }{\log N\hat{\lambda}} + \frac{\tr(\Hb)}{\hat{\lambda}}\right) \exp \bigg(-\frac{1}{\tr(\Hb)} N \frac{1}{\beta}\bigg) \right)^2  \label{eq:sgd_bias_3} \\
   \shortintertext{subsitute $\beta$ in (\ref{eq:sgd_bias_3}), we get:} 
      &=  \mathrm{RidgeBiasBound}[i]  \left( \frac{\lambda_i  }{\log N\hat{\lambda}} + \frac{\tr(\Hb)}{N \hat{\lambda}}  \right)^2 \notag   \\
\shortintertext{by premise, we can obtain that} 
     & \lesssim \mathrm{RidgeBiasBound}[i] \notag
\end{align}

\dz{Eq B/22 seems not correct, we should get a lower bound for $\tilde\lambda_i$, the bound in B.22 cannot be proved via the choice of $\beta$. How (B.23) leads to (B.24) should be clearer. When mentioning "substitute $\eta$ and $\beta$", please give the corresponding equation references.}

% \begin{align}\label{eq:bias}
%     \mathrm{SGDBiasBound[i]} &= (\tilde{\wb}^*[i])^2\frac{1}{N^2 \eta ^2\tilde{\lambda}_i}\exp \bigg(-2\eta N\tilde{\lambda}_i\bigg)  \\
%      &= \tilde{\wb}^*[i]\frac{\tr(\tilde{\Hb})^2}{N^2\tilde{\lambda}_i}\exp \bigg(-\frac{2N\tilde{\lambda}_i}{\tr(\tilde{\Hb})}\bigg)\\
%      & \simeq  \wb^*[i]^2\frac{N^2 \lambda_i^2}{\log(N)^2 \tr(\Hb)^2} \frac{\tr(\Hb)^2}{N^2 \lambda_i} \exp \bigg(-\frac{2N}{\tr(\Hb)} \cdot \frac{\log(N) \tr(\Hb)}{N} \bigg) \\
%      & = \wb^*[i]^2 \frac{\tilde{\lambda}^2}{\lambda_i N^2} \frac{\lambda_i^2}{\log(N)^2 \tilde{\lambda}^2}   \\
%      & = \mathrm{RidgeBias}[i] \frac{\lambda_i^2}{\log(N)^2 \tilde{\lambda}^2} \\
%      & \leq \mathrm{RidgeBiasBound}[i]
% \end{align}

Therefore, combining the results of the two intervals above, we have that 
$$\mathrm{SGDBiasBound} \lesssim \mathrm{RidgeBiasBoud}$$

Next, let's consider variance.
\begin{align}
        \mathrm{SGDVarianceBound} & = (\sigma^2+\frac{\|\tilde{w}^*\|^2_{\Ib_{0:k^*}}+N\eta \|\tilde{w}^*\|^2_{\tilde{\Hb}_{k^*:\infty}} }{N\eta})\cdot\bigg(\frac{k^*}{N}+N\eta^2\sum_{i>k^*}\tilde{\lambda}_i^2\bigg)\\      
         & = (1+\frac{\|\tilde{w}^*\|^2_{\Ib_{0:k^*}}+N\eta \|\tilde{w}^*\|^2_{\tilde{\Hb}_{k^*:\infty}} }{N\eta \sigma^2})\cdot \sigma^2 \bigg(\frac{k^*}{N}+N\eta^2\sum_{i>k^*}\tilde{\lambda}_i^2\bigg)\\
    \shortintertext{subsititue in $\eta$:}
      & = (1+\frac{\|\tilde{w}^*\|^2_{\Ib_{0:k^*}}+N\eta \|\tilde{w}^*\|^2_{\tilde{\Hb}_{k^*:\infty}} }{N\eta \sigma^2})\cdot \sigma^2 \bigg(\frac{k^*}{N}+\frac{N}{\tr(\tilde{\Hb})}\sum_{i>k^*}\tilde{\lambda}_i^2\bigg)\\
    \shortintertext{substitute the premise of the case $\hat{\lambda} \leq \tr(\tilde{\Hb})$ and the fact that $\beta \lambda_i + 1 \geq 1$: }
    & \lesssim (1+\frac{\|\tilde{w}^*\|^2_{\Ib_{0:k^*}}+N\eta \|\tilde{w}^*\|^2_{\tilde{\Hb}_{k^*:\infty}} }{N\eta \sigma^2})\cdot \sigma^2 \bigg(\frac{k^*}{N}+\frac{N}{\hat{\lambda}}\sum_{i>k^*}\lambda_i^2\bigg)\\
          & = (1+\frac{\|\tilde{w}^*\|^2_{\Ib_{0:k^*}}+N\eta \|\tilde{w}^*\|^2_{\tilde{\Hb}_{k^*:\infty}} }{N\eta \sigma^2})\cdot \mathrm{RidgeVarianceBound}\\
          & \lesssim  \mathrm{RidgeVarianceBound}
\end{align}
Therefore, we have that 
$$ \mathrm{SGDVarianceBound} \lesssim \mathrm{RidgeVarianceBound}$$

Combining all the result above, we have that there exists an $\eta$ such that 
$$ \mathrm{SGDRiskBound} \lesssim \mathrm{RidgeRiskBound}.$$

\end{proof}
