# Supplementary material for: Improving Implicit Regularization of SGD with Preconditioning for Least Square Problems
Source: arXiv:2403.08585 source file (2024-05-26)
Supplement: Supplementary file 2 [file preliminary_analysis3.tex]

\newpage
\section{Analysis of precondition SGD with standard ridge regression}
\jw{add beta only on the portion of eigenvector that are not too large or too small}

Because of the exponential term, it is easy to control the bias of SGD with a large enough $N$. The key challenge in the analysis resides in controlling the varaicne of SGD. Now that we do not have the freedom on using difference in sample samplexity, how to use the learning rate $\eta$ and the $\beta$ in the precondition matrix to control the gap of variance between SGD and ridge.

For the preliminary analysis, we consider the case $\Mb = \Ib$ and $\Gb = (\Hb + \beta \Ib)^{-1}$. The goal is to find a $\beta$ for $\Gb$ and a learning rate $\eta$,
$$\mathrm{SGDRisk} \lesssim \mathrm{RidgeRisk}$$

$\Mb = \Ib$ reduces the precondition ridge regression back to the standard case with the following risk bound,

\begin{equation}
    \begin{split}
        \mathrm{RidgeRisk}
\gtrsim \underbrace{\frac{\hat{\lambda}^2}{ N^2}\cdot\big\|\wb^*\big\|_{\Hb_{0:k^*}^{-1}}^2 + \|\wb^*\big\|_{\Hb_{k^*:\infty}}^2}_{\mathrm{RidgeBiasBound}} 
 + \underbrace{\sigma^2\cdot\bigg(\frac{k^*}{N}+\frac{N}{\hat{\lambda}^2}\sum_{i>k^*}\lambda_i^2\bigg)}_{\mathrm{RidgeVarianceBound}},
    \end{split}
\end{equation}

where $\hat{\lambda} = \lambda + \sum_{i>k^*}\lambda_i$. 
Recall that the SGD risk is given by the following, 

\begin{equation}
    \begin{split}
        \mathrm{SGDRisk}
\lesssim \underbrace{\frac{1}{\eta^2 N^2}\cdot\big\|\exp(-N\eta \tilde{\Hb})\tilde{\wb}^*\big\|_{\Hb_{0:k^*}^{-1}}^2 + \|\tilde{\wb}^*\big\|_{\Hb_{k^*:\infty}}^2}_{\mathrm{SGDBiasBound}} \\
+ \underbrace{(\sigma^2+\frac{\|\tilde{w}^*\|^2_{\Ib_{0:k_2}}+N\eta \|\tilde{w}^*\|^2_{\tilde{\Hb}_{k_2:\infty}} }{N\eta})\cdot\bigg(\frac{k_2}{N}+N\eta^2\sum_{i>k_2}\tilde{\lambda}_i^2\bigg)}_{\mathrm{SGDVarianceBound}}.
    \end{split}
\end{equation}

Suppose $\frac{1}{\hat{\lambda}} \leq \frac{1}{ \tr(\tilde{\Hb})}$ is a feasible learning rate. Then setting $\eta = \frac{1}{\hat{\lambda}}$, we have that,

\begin{equation}
    \begin{split}
        \mathrm{SGDBiasBound} & = \frac{1}{\eta^2 N^2}\cdot\big\|\exp(-N\eta \tilde{\Hb})\tilde{\wb}^*\big\|_{\tilde{\Hb}_{0:k^*}^{-1}}^2 + \|\tilde{\wb}^*\big\|_{\tilde{\Hb}_{k^*:\infty}}^2 \\
        &\leq \frac{\hat{\lambda}^2}{N^2} \cdot\big\|\exp(-N\eta \tilde{\Hb})\tilde{\wb}^*\big\|_{\tilde{\Hb}_{0:k^*}^{-1}}^2 + \|\wb^*\big\|_{\Hb_{k^*:\infty}}^2\\
        &\leq \frac{\hat{\lambda}^2}{N^2} \cdot\big\|\exp(-N\eta \tilde{\Hb})\big\|^2 \big\| \wb^*\big\|_{\Hb_{0:k^*}^{-1}}^2 + \|\wb^*\big\|_{\Hb_{k^*:\infty}}^2\\
        &\leq  \frac{\hat{\lambda}^2}{ N^2}\cdot\big\|\wb^*\big\|_{\Hb_{0:k^*}^{-1}}^2 + \|\wb^*\big\|_{\Hb_{k^*:\infty}}^2 \\ 
        &= \mathrm{RidgeBiasBound}
    \end{split}
\end{equation}

Now let's consider the variance, 

\begin{equation}
    \begin{split}
        \mathrm{SGDVarianceBound} & =(\sigma^2+\frac{\|\tilde{w}^*\|^2_{\Ib_{0:k_2}}+N\eta \|\tilde{w}^*\|^2_{\tilde{\Hb}_{k_2:\infty}} }{N\eta})\cdot\bigg(\frac{k_2}{N}+N\eta^2\sum_{i>k_2}\tilde{\lambda}_i^2\bigg)\\
         & =(\sigma^2+\frac{\|\tilde{w}^*\|^2_{\Ib_{0:k_2}}}{N\eta}+ \|\tilde{w}^*\|^2_{\tilde{\Hb}_{k_2:\infty}})\cdot\bigg(\frac{k_2}{N}+N\eta^2\sum_{i>k_2}\tilde{\lambda}_i^2\bigg)\\
          & =(\sigma^2+\frac{\|\tilde{w}^*\|^2_{\Ib_{0:k_2}}\hat{\lambda}}{N }+ \|\tilde{w}^*\|^2_{\tilde{\Hb}_{k_2:\infty}})\cdot\bigg(\frac{k_2}{N}+\frac{N}{\tilde{\lambda}^2}\sum_{i>k_2}\tilde{\lambda}_i^2\bigg)\\
    \end{split}
\end{equation}

We can set $k_2 = k^*_{\mathrm{ridge}}$ and $\Gb[i] = \Ib, \forall i >  k^*_{\mathrm{ridge}} $, we have

\begin{equation}
    \begin{split}
        \mathrm{SGDVarianceBound} & (\sigma^2+\frac{\|\tilde{w}^*\|^2_{\Ib_{0:k^*_{\mathrm{ridge}}}}\hat{\lambda}}{N }+ \|\tilde{w}^*\|^2_{\tilde{\Hb}_{k^*_{\mathrm{ridge}}:\infty}})\cdot\bigg(\frac{k^*_{\mathrm{ridge}}}{N}+\frac{N}{\tilde{\lambda}^2}\sum_{i>k^*_{\mathrm{ridge}}}\lambda_i^2\bigg)\\
    \end{split}
\end{equation}

Based on the fact that $\hat{\lambda}$ is a constant, we have that 
$$\|\tilde{w}^*\|^2_{\tilde{\Hb}_{k^*_{\mathrm{ridge}}:\infty}} = \|{w}^*\|^2_{{\Hb}_{k^*_{\mathrm{ridge}}:\infty}} \leq \hat{\lambda} \lesssim \theta(1)$$

Then it remains to show that 
$$\frac{\|\tilde{w}^*\|^2_{\Ib_{0:k^*_{\mathrm{ridge}}}}\hat{\lambda}}{N } \lesssim \theta(1)$$

\jw{This seems to trivially hold as $\hat{\lambda}$ is a constant and $\|\tilde{w}^*\|^2_{\Ib_{0:k^*_{\mathrm{ridge}}}}$ is finite}

Therefore, we have $$\mathrm{SGDVarianceBound} \lesssim \mathrm{RidgeVarianceBound}.$$

\jw{One easy route from here is to tune $\Gb$ so that $\frac{1}{\hat{\lambda}} \leq \frac{1}{ \tr(\tilde{\Hb})}$ always holds. }

This leads to 
\begin{equation}
    \begin{split}
        \frac{1}{\hat{\lambda}} & \leq \frac{1}{ \tr(\tilde{\Hb})}\\
         \tr(\tilde{\Hb}) & \leq \hat{\lambda} \\
          \tr(\tilde{\Hb})  &\leq \lambda + \sum_{i > k^*_{\mathrm{ridge}}} \lambda_i \\
    \end{split}
\end{equation}
Based on the proof, we need to set $\tilde{\lambda_i} = \lambda_i, \text{ for } i >  k^*_{\mathrm{ridge}}$. Therefore, to satisfy the above inequality, we need
\begin{equation}
    \begin{split}
        \lambda & \geq \sum_{i \leq k^*_{\mathrm{ridge}}} \tilde{\lambda_i} \\
        \lambda & \geq \sum_{i \leq k^*_{\mathrm{ridge}}} \frac{\lambda_i}{\lambda_i + \beta}  \geq  \frac{k^*_{\mathrm{ridge}} \lambda_{k^*_{\mathrm{ridge}}}}{\lambda_{k^*_{\mathrm{ridge}}} + \beta} \\
        \beta & \geq \lambda_{k^*_{\mathrm{ridge}}} (\lambda k^*_{\mathrm{ridge}} - 1)
    \end{split}
\end{equation}

\jw{The following analysis is still loose at the moment}

Suppose $\hat{\lambda} > \alpha \tr(\tilde{\Hb})$, we set the learning rate to be largest possible $\eta = \frac{1}{\alpha \tr(\tilde{\Hb})}$,

\begin{equation}
    \begin{split}
        \mathrm{SGDBiasBound}  &\le \frac{(1-\eta\lambda_{k^*})^{2N}}{\eta^2N^2}\cdot \|\tilde{\wb}^*\|_{\tilde{\Hb}_{0:k^*}}^2 + \|\tilde{\wb}^*\|_{\tilde{\Hb}_{k^*:\infty}}^2\notag\\
    \end{split}
\end{equation}

Because $1-\eta\lambda_{k^*} < 1$, we have 
\begin{equation}
    \begin{split}
     \frac{(1-\eta\lambda_{k^*})^{2N}}{{\eta^2N^2}} /\frac{\hat{\lambda}^2}{ N^2}  \\
     = \frac{(1-\eta\lambda_{k^*})^{2N}}{\hat{\lambda}^2 \eta^2} \\
    \end{split}
\end{equation}
$$\frac{(1-\eta\lambda_{k^*})^{2N}}{\hat{\lambda}^2 \eta^2} 
     \mapsto 0,  N \mapsto \infty$$

Therefore, for a large enough $N$, we have 
\begin{equation}
    \begin{split}
        \mathrm{SGDBiasBound}  &\le \frac{(1-\eta\lambda_{k^*})^{2N}}{\eta^2N^2}\cdot \|\tilde{\wb}^*\|_{\tilde{\Hb}_{0:k^*}}^2 + \|\tilde{\wb}^*\|_{\tilde{\Hb}_{k^*:\infty}}^2\notag\\
         &\leq  \frac{\hat{\lambda}}{ N^2}\cdot\big\|\wb^*\big\|_{\Hb_{0:k^*}^{-1}}^2 + \|\wb^*\big\|_{\Hb_{k^*:\infty}}^2 \\ 
        &= \mathrm{RidgeBiasBound}
    \end{split}
\end{equation}

Now, we continue to show the variance,

\begin{equation}
    \begin{split}
        \mathrm{SGDVarianceBound} & =(1+R^2)\sigma^2\cdot\bigg(\frac{k^*}{N}+\frac{N}{\eta^2}\sum_{i>k^*}\tilde{\lambda}_i^2\bigg) \\
        & =(1+R^2)\sigma^2\cdot\bigg(\frac{k^*}{N}+\frac{N}{\eta^2}\sum_{i>k^*}\frac{{\lambda_i}^2}{(\lambda_i+\beta)^2}\bigg) \\
        & \leq (1+R^2)\sigma^2\cdot\bigg(\frac{k^*}{N}+\frac{N}{\eta^2 \beta^2}\sum_{i>k^*}{\lambda}_i^2 \bigg) 
    \end{split}
\end{equation}

Therefore, so long as we have 
% \begin{equation}
%     \begin{split}
%         \frac{N}{\eta^2 \beta^2} & \leq \frac{1}{\hat{\lambda}^2}\\
%         \beta^2 & \geq \frac{\hat{\lambda}^2N}{\eta^2}
%     \end{split}
% \end{equation}

\begin{equation}
    \begin{split}
        \frac{1}{\eta^2 (\lambda_i + \beta)^2} & \leq \frac{1}{\hat{\lambda}^2}\\
        (\lambda_i + \beta)^2 & \geq \frac{\hat{\lambda}^2}{\eta^2}
    \end{split}
\end{equation}

We get that

\begin{equation}
    \begin{split}
        \mathrm{SGDVarianceBound} 
        & \leq (1+R^2)\sigma^2\cdot\bigg(\frac{k^*}{N}+\frac{N}{\eta^2 \beta^2}\sum_{i>k^*}{\lambda}_i^2 \bigg) \\
        & \leq (1+R^2)\sigma^2\cdot\bigg(\frac{k^*}{N}+\frac{N}{\hat{\lambda}^2}\sum_{i>k^*}{\lambda}_i^2 \bigg)\\
        & = (1+R^2) \mathrm{RidgeVarianceBound}
      \end{split}
\end{equation}

\jw{There are different versions of risk bound for both SGD and Ridge used in the note and the paper. I am not quite sure if they are equivalent. If not,  when can I use one not the other?}

\jw{Is the $\alpha$ factor a typo in the note? I am not sure where $\alpha$ in Theorem~\ref{theorem:precondition_sgd_fit} comes from.  What does $\alpha$ depends on, what the ranges is or what are the constraint. }

\jw{$\lesssim$ seems to be a pretty loss bound? does not need to do much on the precondition matrix $G$. When can we ignore some constant?}

\jw{I do not quite get why there are three intervals in the note? My guest is $[0,k_{\mathrm{ridge}}^*],[k_{\mathrm{ridge}}^*,N],[N, \infty]$}

\jw{How strong is the requirement for ``same'' sample size? exactly the same? or in the same order?}

\jw{There are quite some steps in the proof missing. The result we are seeking is closest to Theorem 5.3 in ~\citep{zou2021benefits}. There are quite some steps I can not follow in the proof for Theorem 5.3.}
