# Supplementary material for: Improving Implicit Regularization of SGD with Preconditioning for Least Square Problems
Source: arXiv:2403.08585 source file (2024-05-26)
Supplement: Supplementary file 3 [file preliminary_analysis4.tex]

\newpage
\section{Analysis of precondition SGD with standard ridge regression}
\jw{tune $\tilde{\Hb}$ so that $\tilde{\lambda_i} = \lambda_{k^*} \text{ for } i \leq k^*$}

The goal is to utilize the exponential term in the SGD bias along with the preconditioning to control the bias term of SGD. We can leave some constant factor difference in term of signal to noise ratio in the variance term.

For the preliminary analysis, we consider the case $\Mb = \Ib$ and $\Gb = (\Hb + \beta \Ib)^{-1}$. The goal is to find a $\beta$ for $\Gb$ and a learning rate $\eta$ such that,
$$\mathrm{SGDRisk} \lesssim \mathrm{RidgeRisk}.$$

$\Mb = \Ib$ reduces the precondition ridge regression back to the standard case with the following risk bound,

\begin{equation}
    \begin{split}
        \mathrm{RidgeRisk}
\gtrsim \underbrace{\frac{\hat{\lambda}^2}{ N^2}\cdot\big\|\wb^*\big\|_{\Hb_{0:k^*_{\mathrm{Ridge}}}^{-1}}^2 + \|\wb^*\big\|_{\Hb_{k^*_{\mathrm{Ridge}}:\infty}}^2}_{\mathrm{RidgeBiasBound}} 
 + \underbrace{\sigma^2\cdot\bigg(\frac{k^*_{\mathrm{Ridge}}}{N}+\frac{N}{\hat{\lambda}^2}\sum_{i>k^*_{\mathrm{Ridge}}}\lambda_i^2\bigg)}_{\mathrm{RidgeVarianceBound}},
    \end{split}
\end{equation}

where 
$$\hat{\lambda} = \lambda + \sum_{i>k^*}\lambda_i$$ 
and 
$$k^*_{\mathrm{Ridge}} := \min\{k: b\lambda_{k} \leq \frac{\lambda + \sum_{i >k}\lambda_i}{N}\}.$$ 
Recall that the SGD risk is given by the following,

\begin{equation}
    \begin{split}
        \mathrm{SGDRisk}
\lesssim \underbrace{\frac{1}{\eta^2 N^2}\cdot\big\|\exp(-N\eta \tilde{\Hb})\tilde{\wb}^*\big\|_{\Hb_{0:k_1}^{-1}}^2 + \|\tilde{\wb}^*\big\|_{\Hb_{k_1:\infty}}^2}_{\mathrm{SGDBiasBound}} \\
+ \underbrace{(\sigma^2+\frac{\|\tilde{w}^*\|^2_{\Ib_{0:k_2}}+N\eta \|\tilde{w}^*\|^2_{\tilde{\Hb}_{k_2:\infty}} }{N\eta})\cdot\bigg(\frac{k_2}{N}+N\eta^2\sum_{i>k_2}\tilde{\lambda}_i^2\bigg)}_{\mathrm{SGDVarianceBound}}.
    \end{split}
\end{equation}
for arbitrary $k_1,k_2 \in [d]$.

Suppose $\frac{1}{\hat{\lambda}} \leq \frac{1}{ \tr(\tilde{\Hb})}$ is a feasible learning rate. 

Then setting $\eta = \frac{1}{\hat{\lambda}}$ and $k_1 = k^*_{\mathrm{Ridge}}$, we have that,
\begin{equation}
    \begin{split}
        \mathrm{SGDBiasBound} & = \frac{1}{\eta^2 N^2}\cdot\big\|\exp(-N\eta \tilde{\Hb})\tilde{\wb}^*\big\|_{\tilde{\Hb}_{0:k^*_{\mathrm{Ridge}}}^{-1}}^2 + \|\tilde{\wb}^*\big\|_{\tilde{\Hb}_{k^*_{\mathrm{Ridge}}:\infty}}^2 \\
        &\leq \frac{\hat{\lambda}^2}{N^2} \cdot\big\|\exp(-N\eta \tilde{\Hb})\tilde{\wb}^*\big\|_{\tilde{\Hb}_{0:k^*_{\mathrm{Ridge}}}^{-1}}^2 + \|\wb^*\big\|_{\Hb_{k^*_{\mathrm{Ridge}}:\infty}}^2\\
        &\leq \frac{\hat{\lambda}^2}{N^2} \cdot\big\|\exp(-N\eta \tilde{\Hb})\big\|^2 \big\| \tilde{\wb}^*\big\|_{\tilde{\Hb}_{0:k^*}^{-1}}^2 + \|\wb^*\big\|_{\Hb_{k^*:\infty}}^2\\
        &\leq  \frac{\hat{\lambda}^2}{ N^2}\cdot\big\|\tilde{\wb}^*\big\|_{\tilde{\Hb}_{0:k^*}^{-1}}^2 + \|\wb^*\big\|_{\Hb_{k^*:\infty}}^2 \\ 
        &\leq  \frac{\hat{\lambda}^2}{ N^2}\cdot\big\|\wb^*\big\|_{{\Hb}_{0:k^*}^{-1}}^2 + \|\wb^*\big\|_{\Hb_{k^*:\infty}}^2 \\ 
        &= \mathrm{RidgeBiasBound}
    \end{split}
\end{equation}

Suppose $\hat{\lambda} \leq \tr(\tilde{\Hb})$, i.e., $\frac{1}{\hat{\lambda}}$ is no longer a feasible learning rate. We set $\eta = \tr(\tilde{\Hb})$ to be the largest possible learning rate. Similarly, we set $k_1 = k^*_{\mathrm{Ridge}}$, and we have that,

\begin{equation}
    \begin{split}
        \mathrm{SGDBiasBound} & = \frac{1}{\eta^2 N^2}\cdot\big\|\exp(-N\eta \tilde{\Hb})\tilde{\wb}^*\big\|_{\tilde{\Hb}_{0:k^*_{\mathrm{Ridge}}}^{-1}}^2 + \|\tilde{\wb}^*\big\|_{\tilde{\Hb}_{k^*_{\mathrm{Ridge}}:\infty}}^2 \\
        &\leq \frac{\tr(\tilde{\Hb})^2}{N^2} \cdot\big\|\exp(-N\eta \tilde{\Hb})\tilde{\wb}^*\big\|_{\tilde{\Hb}_{0:k^*_{\mathrm{Ridge}}}^{-1}}^2 + \|\wb^*\big\|_{\Hb_{k^*_{\mathrm{Ridge}}:\infty}}^2\\
        &\leq \frac{\tr(\tilde{\Hb})^2}{N^2} \cdot\big\|\exp(-N\eta \tilde{\Hb})\big\|^2 \big\| \tilde{\wb}^*\big\|_{\tilde{\Hb}_{0:k^*}^{-1}}^2 + \|\wb^*\big\|_{\Hb_{k^*:\infty}}^2\\
        &= \frac{\tr(\tilde{\Hb})^2}{N^2} \cdot \sum_{i < k^*}\big\|\exp(-N\eta \tilde{\lambda_{i}})\big\|^2  \tilde{\wb}^*[i]^2/\tilde{\lambda_i} + \|\wb^*\big\|_{\Hb_{k^*:\infty}}^2\\
    \end{split}
\end{equation}

Since the second term in the expression above matches perfectly with RidgeBiasBound. Therefore, to show 
$$\mathrm{SGDBiasBound} \lesssim \mathrm{RidgeBiasBound},$$
it is enough to show that,
\begin{equation}
    \begin{split}
        \frac{\tr(\tilde{\Hb})^2}{N^2} \cdot \sum_{i < k^*}\big\|\exp(-N\eta \tilde{\lambda_{i}})\big\|^2  \tilde{\wb}^*[i]^2/\tilde{\lambda_i} \leq \frac{\hat{\lambda}^2}{ N^2}\cdot\big\|\wb^*\big\|_{\Hb_{0:k^*_{\mathrm{Ridge}}}^{-1}}^2.
    \end{split}
\end{equation}

\begin{equation}
    \begin{split}
         \frac{\tr(\tilde{\Hb})}{N} \cdot  \exp(-N\eta \tilde{\lambda_{i}})  \tilde{\wb}^*[i]/\tilde{\lambda}_i^{1/2} & = \frac{1}{N}\big( \sum_{i \leq k^*_{\mathrm{Ridge}}} \tilde{\lambda_i} + \sum_{i > k^*_{\mathrm{Ridge}}} \lambda_i \big) \exp(-\frac{N \tilde{\lambda_{i}}}{\tr(\tilde{\Hb})}) \tilde{\wb}^*[i]/\tilde{\lambda}_i^{1/2}\\ 
         & = \frac{\lambda_i + \beta_i}{N}\big(k^*_{\mathrm{Ridge}} \tilde{\lambda}_{k^*_{\mathrm{Ridge}}} + \sum_{i > k^*_{\mathrm{Ridge}}} \lambda_i \big) \exp(-\frac{N \tilde{\lambda_{i}}}{\tr(\tilde{\Hb})}) {\wb}^*[i]/{\lambda}_i^{1/2}\\
    \end{split}
\end{equation}
