# Supplementary material for: Improving Implicit Regularization of SGD with Preconditioning for Least Square Problems
Source: arXiv:2403.08585 source file (2024-05-26)
Supplement: Supplementary file 4 [file lemma_eigenvalue.tex]

\begin{lemma}
    Suppose $\Gb = \Hb + \beta \Ib$, then $\tilde{\Hb} = \Gb^{1/2} \Hb \Gb^{1/2}$ have same eigenvectors as $\Hb$ with eigenvalues $\tilde{\lambda}_i = \lambda_i(\lambda_i + \beta)$ 
\end{lemma}

\begin{lemma}
    Suppose $\Gb = (\Hb + \beta \Ib)^{-1}$, then $\tilde{\Hb} = \Gb^{1/2} \Hb \Gb^{1/2}$ have same eigenvectors as $\Hb$ with eigenvalues $\tilde{\lambda}_i = \lambda_i(\lambda_i + \beta)^{-1}$ 
\end{lemma}

\begin{lemma}
    Suppose $\Mb = \Hb + \lambda \Ib$, then $\hat{\Hb} =\Hb^{1/2}\Mb^{-1}\Hb^{1/2}$ have same eigenvectors as $\Hb$ with eigenvalues $\hat{\lambda}_i = \lambda_i(\lambda_i + \lambda)^{-1}$ 
\end{lemma}

\begin{lemma}
  $ \tr( \Gb^{1/2} \Hb \Gb^{1/2}) = \tr(\Gb \Hb)$
\end{lemma}
