# Supplementary material for: Improving Implicit Regularization of SGD with Preconditioning for Least Square Problems
Source: arXiv:2403.08585 source file (2024-05-26)
Supplement: Supplementary file 6 [file lemma_matrix_norm.tex]

\begin{lemma}\label{lemma:double_effect}
    For all choice of $\Gb$, we have $\|\tilde{\wb}^*\big\|_{\tilde{\Hb}}^2 = \|\wb^*\big\|_{\Hb}^2$.
\end{lemma}

\begin{coro}
 We have $R^2 = \|\wb^*\big\|_{\Hb}^2 / \sigma^2 =  \|\tilde{\wb}^*\big\|_{\tilde{\Hb}}^2 / \sigma^2 $. In other words, changing the precondition matrix $\Gb$ does not affect ``signal to noise'' ratio.
\end{coro}

\begin{lemma}
    For all choice of $\Mb$, we have $\|\hat{\wb}^*\big\|_{\hat{\Hb}}^2 = \|\wb^*\big\|_{\Hb}^2$.
\end{lemma}
