# Supplementary material for: Improving Implicit Regularization of SGD with Preconditioning for Least Square Problems
Source: arXiv:2403.08585 source file (2024-05-26)
Supplement: Supplementary file 7 [file lr_tune.tex]

\newpage
\section{Analysis of precondition SGD with standard ridge regression}

\begin{theorem}[learning rate tune]
Suppose 
$$\Gb[i] = \frac{\lambda}{k^*_{\mathrm{ridge    }}}, \quad \forall i \leq \lambda_{k^*_{\mathrm{ridge}}},$$
$$\Gb[i] = \Ib, \mathrm{otherwise}.$$

Let $\wb_{\mathrm{sgd}}(N, \Gb; \gamma)$ and $\wb_{\mathrm{ridge}}(N; \lambda)$ be the solutions found by the pre-conditioned SGD and ridge regression respectively. Then under Assumption~\ref{}, for any least square problem instance such that the ridge regression solution is generalizable  and any $\lambda$, there exists a choice of stepsize $\gamma^*$ for precondiition-SGD such that
% Then for every problem instance that satisfies Assumption \ref{assump:data_distribution}, and every ridge regression solution in the generalizable regime, there exists a choice of stepsize $\gamma^*$ for SGD such that
\begin{align*}
L\big[\wb_{\mathrm{sgd}}(N, \Gb; \gamma^*)\big]-L(\wb^*)\lesssim L\big[\wb_{\mathrm{ridge}}(N;\lambda)\big] -L(\wb^*),
\end{align*}
\end{theorem}

\begin{proof}
First recall the risk bound of ridge regression,

\begin{equation}
    \begin{split}
        \mathrm{RidgeRisk}
\gtrsim \underbrace{\frac{\hat{\lambda}^2}{ N^2}\cdot\big\|\wb^*\big\|_{\Hb_{0:k^*}^{-1}}^2 + \|\wb^*\big\|_{\Hb_{k^*:\infty}}^2}_{\mathrm{RidgeBiasBound}} 
 + \underbrace{\sigma^2\cdot\bigg(\frac{k^*}{N}+\frac{N}{\hat{\lambda}^2}\sum_{i>k^*}\lambda_i^2\bigg)}_{\mathrm{RidgeVarianceBound}},
    \end{split}
\end{equation}

where $\hat{\lambda} = \lambda + \sum_{i>k^*}\lambda_i$. 

Recall that the SGD risk is given by the following, 

\begin{equation}
    \begin{split}
        \mathrm{SGDRisk}
\lesssim \underbrace{\frac{1}{\eta^2 N^2}\cdot\big\|\exp(-N\eta \tilde{\Hb})\tilde{\wb}^*\big\|_{\Hb_{0:k^*}^{-1}}^2 + \|\tilde{\wb}^*\big\|_{\Hb_{k^*:\infty}}^2}_{\mathrm{SGDBiasBound}} \\
+ \underbrace{(\sigma^2+\frac{\|\tilde{w}^*\|^2_{\Ib_{0:k_2}}+N\eta \|\tilde{w}^*\|^2_{\tilde{\Hb}_{k_2:\infty}} }{N\eta})\cdot\bigg(\frac{k_2}{N}+N\eta^2\sum_{i>k_2}\tilde{\lambda}_i^2\bigg)}_{\mathrm{SGDVarianceBound}}.
    \end{split}
\end{equation}

$$k^*_{\mathrm{ridge}} := \min\{k: b\lambda_{k} \leq \frac{\lambda + \sum_{i >k}\lambda_i}{N}\}.$$ 

\begin{equation}
    \begin{split}
       \tr(\tilde{\Hb}) &= \sum_{i \leq k^*_{\mathrm{ridge}}} \tilde{\lambda}_i +  \sum_{i > k^*_{\mathrm{ridge}}} \lambda_i \\
       & \leq k^*_{\mathrm{ridge}} \frac{\lambda}{k^*_{\mathrm{ridge }}} + \sum_{i > k^*_{\mathrm{ridge}}} \lambda_i \\
       & = \hat{\lambda}
    \end{split}
\end{equation}

This means that we have $\frac{1}{\hat{\lambda}} \leq \frac{1}{ \tr(\tilde{\Hb})}$, and  $\frac{1}{\hat{\lambda}} $ is a feasible learning rate. Then setting $\eta = \frac{1}{\hat{\lambda}}$, we have that,

\begin{equation}
    \begin{split}
        \mathrm{SGDBiasBound} & = \frac{1}{\eta^2 N^2}\cdot\big\|\exp(-N\eta \tilde{\Hb})\tilde{\wb}^*\big\|_{\tilde{\Hb}_{0:k^*}^{-1}}^2 + \|\tilde{\wb}^*\big\|_{\tilde{\Hb}_{k^*:\infty}}^2 \\
        &\leq \frac{\hat{\lambda}^2}{N^2} \cdot\big\|\exp(-N\eta \tilde{\Hb})\tilde{\wb}^*\big\|_{\tilde{\Hb}_{0:k^*}^{-1}}^2 + \|\wb^*\big\|_{\Hb_{k^*:\infty}}^2\\
        &\leq \frac{\hat{\lambda}^2}{N^2} \cdot\big\|\exp(-N\eta \tilde{\Hb})\big\|^2 \big\| \wb^*\big\|_{\Hb_{0:k^*}^{-1}}^2 + \|\wb^*\big\|_{\Hb_{k^*:\infty}}^2\\
        &\leq  \frac{\hat{\lambda}^2}{ N^2}\cdot\big\|\wb^*\big\|_{\Hb_{0:k^*}^{-1}}^2 + \|\wb^*\big\|_{\Hb_{k^*:\infty}}^2 \\ 
        &= \mathrm{RidgeBiasBound}
    \end{split}
\end{equation}

Now let's consider the variance, 

\begin{equation}
    \begin{split}
        \mathrm{SGDVarianceBound} & =(\sigma^2+\frac{\|\tilde{w}^*\|^2_{\Ib_{0:k_2}}+N\eta \|\tilde{w}^*\|^2_{\tilde{\Hb}_{k_2:\infty}} }{N\eta})\cdot\bigg(\frac{k_2}{N}+N\eta^2\sum_{i>k_2}\tilde{\lambda}_i^2\bigg)\\
         & =(\sigma^2+\frac{\|\tilde{w}^*\|^2_{\Ib_{0:k_2}}}{N\eta}+ \|\tilde{w}^*\|^2_{\tilde{\Hb}_{k_2:\infty}})\cdot\bigg(\frac{k_2}{N}+N\eta^2\sum_{i>k_2}\tilde{\lambda}_i^2\bigg)\\
          & =(\sigma^2+\frac{\|\tilde{w}^*\|^2_{\Ib_{0:k_2}}\hat{\lambda}}{N }+ \|\tilde{w}^*\|^2_{\tilde{\Hb}_{k_2:\infty}})\cdot\bigg(\frac{k_2}{N}+\frac{N}{\tilde{\lambda}^2}\sum_{i>k_2}\tilde{\lambda}_i^2\bigg)\\
    \end{split}
\end{equation}

We can set $k_2 = k^*_{\mathrm{ridge}}$ and $\Gb[i] = \Ib, \forall i >  k^*_{\mathrm{ridge}} $, we have

\begin{equation}
    \begin{split}
        \mathrm{SGDVarianceBound} & \leq0.
        (\sigma^2+\frac{\|\tilde{w}^*\|^2_{\Ib_{0:k^*_{\mathrm{ridge}}}}\hat{\lambda}}{N }+ \|\tilde{w}^*\|^2_{\tilde{\Hb}_{k^*_{\mathrm{ridge}}:\infty}})\cdot\bigg(\frac{k^*_{\mathrm{ridge}}}{N}+\frac{N}{\hat{\lambda}^2}\sum_{i>k^*_{\mathrm{ridge}}}\lambda_i^2\bigg)\\
    \end{split}
\end{equation}

Based on the fact that $\hat{\lambda}$ is a constant, we have that 
$$\|\tilde{w}^*\|^2_{\tilde{\Hb}_{k^*_{\mathrm{ridge}}:\infty}} = \|{w}^*\|^2_{{\Hb}_{k^*_{\mathrm{ridge}}:\infty}} \leq \hat{\lambda} \lesssim \theta(1)$$

Then it remains to show that 
$$\frac{\|\tilde{w}^*\|^2_{\Ib_{0:k^*_{\mathrm{ridge}}}}\hat{\lambda}}{N } \lesssim \theta(1)$$

% \jw{This seems to trivially hold as $\hat{\lambda}$ is a constant and $\|\tilde{w}^*\|^2_{\Ib_{0:k^*_{\mathrm{ridge}}}}$ is finite}

Therefore, we have $$\mathrm{SGDVarianceBound} \lesssim \mathrm{RidgeVarianceBound}.$$

\end{proof}
