# Supplementary material for: Improving Implicit Regularization of SGD with Preconditioning for Least Square Problems
Source: arXiv:2403.08585 source file (2024-05-26)
Supplement: Supplementary file 8 [file meeting.tex]

\section{Note for the Meeting}
To specify an instance of SGD,
$$\mathrm{SGD} = (\Hb,\wb^*,\eta,N_s)$$

To specify an instance of Ridge,
$$\mathrm{SGD} = (\Hb,\wb^*,\lambda,N_r)$$

In ~\citep{zou2021benefits}, it is established that 

\begin{enumerate}
    \item Under certain data distributions (one-hot and Gaussian), the risk bound of SGD is no worse than Ridge when given a larger sample size. 
\end{enumerate}

{\bf GOAL:} We want to show that for a proper choice of precondition matrix $\Gb$, pre-condition SGD can perform no worse than Ridge when given ``same'' sample size.

\begin{enumerate}
    \item \jw{There are different versions of risk bound for both SGD and Ridge used in the paper. I am not quite sure if they are equivalent. If not,  when can I use one not the other?}
    \item \jw{There are quite some steps in the proof missing.}
    \item \jw{How strong is the requirement for ``same'' sample size? exactly the same? or at the same order?}
    \item \jw{$\lesssim$ seems to be a pretty loss bound? does not need to do much on the precondition matrix $G$.}
\end{enumerate}
