# Supplementary material for: Improving Implicit Regularization of SGD with Preconditioning for Least Square Problems
Source: arXiv:2403.08585 source file (2024-05-26)
Supplement: Supplementary file 9 [file precond_sgd_outperformance_precond_ridge.tex]

\newpage
\section{Analysis of preconditioned SGD with preconditioned ridge regression}
\begin{theorem}[preconditioned SGD outperform preconditioned ridge]\label{thm:H_I}
Let $\Mb$ be the given PSD preconditioned matrix for the ridge regression with the same eigenvectors as $\Hb$. Then, let
$$\Gb =  \big ( \beta \Hb + \Ib \big )^{-1},$$
and 
$$\beta = \frac{N}{\log N \tr(\Hb)}$$

Let $\wb_{\mathrm{sgd}}(N, \Gb; \gamma)$ and $\wb_{\mathrm{ridge}}(N; \lambda)$ be the solutions found by the pre-conditioned SGD and ridge regression respectively. Then under Assumption~\ref{assump:fourth_moment},~\ref{assump:model_noise}, for any least square problem instance such that the ridge regression solution is generalizable  and any $\lambda$, there exists a choice of stepsize $\gamma^*$ for preconditioned-SGD such that
% Then for every problem instance that satisfies Assumption \ref{assump:data_distribution}, and every ridge regression solution in the generalizable regime, there exists a choice of stepsize $\gamma^*$ for SGD such that
\begin{align*}
L\big[\wb_{\mathrm{sgd}}(N, \Gb; \gamma^*)\big]-L(\wb^*)\lesssim L\big[\wb_{\mathrm{ridge}}(N;\lambda)\big] -L(\wb^*),
\end{align*}
\end{theorem}

\begin{lemma}\label{lemma:tilde_eigen}
    Suppose $$\Gb = \Mb^{-1} \big ( \beta \Hb + \Ib \big )^{-1},$$
    then we have 
    $$\tilde{\lambda}_i = \frac{1}{\gamma_i}\frac{\lambda_i}{\beta \lambda_i + 1}.$$
\end{lemma}

\begin{lemma}\label{lemma:monotone}
    For $i \in [d-1]$, we have $$\tilde{\lambda}_{i+1} \leq \tilde{\lambda}_{i}.$$
\end{lemma}

\begin{proof}[Proof of Theorem~\ref{thm:H_I}]
By Theorem~\ref{theorem:precondition_ridge_fit}, the learning dynamic of SGD after preconditioning can be characterized by $\tilde{\Hb} = \Gb^{1/2}\Hb\Gb^{1/2}$. By Lemma~\ref{lemma:tilde_eigen}, we can obtain the following eigenspectrum of $\tilde{\Hb}$:
$$\tilde{\lambda}_i = \frac{\lambda_i}{\gamma_i(\beta \lambda_i + 1)}$$
Then recall the lower bound of the risk achieved by ridge regression with parameter $\lambda$ and preconditioned matrix $\Mb$:
\begin{equation}
    \begin{split}
        \mathrm{RidgeRiskBound}
\gtrsim \underbrace{\frac{\hat{\lambda}^2}{ N^2}\cdot\big\|\hat{\wb}^*\big\|_{\hat{\Hb}_{0:k^*}^{-1}}^2 + \|\hat{\wb}^*\big\|_{\hat{\Hb}_{k^*:\infty}}^2}_{\mathrm{RidgeBiasBound}} 
 + \underbrace{\sigma^2\cdot\bigg(\frac{k^*}{N}+\frac{N}{\hat{\lambda}^2}\sum_{i>k^*}\hat{\lambda}_i^2\bigg)}_{\mathrm{RidgeVarianceBound}},
    \end{split}
\end{equation}
where $\hat{\lambda} = \lambda + \sum_{i>k^*}\hat{\lambda}_i$ and $k^* = \min \{k: \hat{\lambda}_k \leq \frac{\lambda + \sum_{i>k}\hat{\lambda}_i}{N}\}$. 

Then recall the upper bound of SGD risk is given by the following, where the parameter $k_1,k_2\in[d]$ can be arbitrarily chosen:
\begin{equation}
    \begin{split}
        \mathrm{SGDRiskBound}
&\lesssim \underbrace{\frac{1}{\eta^2 N^2}\cdot\big\|\exp(-N\eta \tilde{\Hb})\tilde{\wb}^*\big\|_{\tilde{\Hb}_{0:k_1}^{-1}}^2 + \|\tilde{\wb}^*\big\|_{\tilde{\Hb}_{k_1:\infty}}^2}_{\mathrm{SGDBiasBound}} \\
&\qquad + \underbrace{\bigg (\sigma^2+\frac{\|\tilde{\wb}^*\|^2_{\Ib_{0:k_2}}+N\eta \|\tilde{\wb}^*\|^2_{\tilde{\Hb}_{k_2:\infty}} }{N\eta} \bigg)\cdot\bigg(\frac{k_2}{N}+N\eta^2\sum_{i>k_2}\tilde{\lambda}_i^2\bigg)}_{\mathrm{SGDVarianceBound}}.
    \end{split}
\end{equation}

Similarly, we divide the analysis into two cases: {\bf Case I:} $\tilde{\lambda} \geq \tr(\tilde{\Hb})$ and {\bf Case II:} $\tilde{\lambda} < \tr(\tilde{\Hb})$.

For {\bf Case I}, we have that $\frac{1}{\hat{\lambda}} \leq \frac{1}{\tr(\tilde{\Hb})}$. We can set $\eta = \frac{1}{\hat{\lambda}}$ and $k_1,k_2 = k^*$. We divide the analysis into bias and variance. For the bias, we have that,

\begin{align*}
        \mathrm{SGDBiasBound}
& \lesssim \frac{\tilde{\lambda}^2}{ N^2}\cdot\bigg\|\exp(-\frac{N\tilde{\Hb}}{\tilde{\lambda}^2})\tilde{\wb}^*\bigg\|_{\tilde{\Hb}_{0:k^*}^{-1}}^2 + \|\tilde{\wb}^*\big\|_{\tilde{\Hb}_{k^*:\infty}}^2 \\
& \lesssim \frac{\tilde{\lambda}^2}{ N^2}\cdot\bigg\|\exp(-\frac{N\tilde{\Hb}}{\tilde{\lambda}}) \bigg \|^2 \big \| \tilde{\wb}^*\big\|_{{\Hb}_{0:k^*}^{-1}}^2 + \|\tilde{\wb}^*\big\|_{\tilde{\Hb}_{k^*:\infty}}^2 \\
& \lesssim \frac{\tilde{\lambda}^2}{ N^2}\cdot\bigg\|\exp(-\frac{N\tilde{\Hb}}{\tilde{\lambda}}) \bigg \|^2 \big \| {\wb}^*\big\|_{{\Hb}_{0:k^*}^{-1}}^2 + \|{\wb}^*\big\|_{{\Hb}_{k^*:\infty}}^2 \\
& \lesssim \frac{\tilde{\lambda}^2}{ N^2}\cdot \big \| {\wb}^*\big\|_{{\Hb}_{0:k^*}^{-1}}^2 + \|{\wb}^*\big\|_{{\Hb}_{k^*:\infty}}^2 \\
& \lesssim \frac{\tilde{\lambda}^2}{ N^2}\cdot \big \| {\hat{\wb}}^*\big\|_{\hat{\Hb}_{0:k^*}^{-1}}^2 + \|\hat{\wb}^*\big\|_{\hat{\Hb}_{k^*:\infty}}^2 \\
& = \mathrm{RidgeBiasBound}
\end{align*}

For the variance we have, 

\begin{align*}
        \mathrm{SGDVarianceBound}
& \lesssim \bigg (\sigma^2+\frac{\|\tilde{\wb}^*\|^2_{\Ib_{0:k^*}}+N\eta \|\tilde{\wb}^*\|^2_{\tilde{\Hb}_{k^*:\infty}} }{N\eta}\bigg)\cdot\bigg(\frac{k^*}{N}+N\eta^2\sum_{i>k^*}\tilde{\lambda}_i^2\bigg) \\
 & \lesssim \Theta(1)\cdot \sigma^2 \bigg(\frac{k^*}{N}+\frac{N}{\hat{\lambda}^2}\sum_{i>k^*}\tilde{\lambda}_i^2\bigg)\\
\shortintertext{using the fact that $\tilde{\lambda}_i = \frac{\lambda_i}{\gamma_i(\beta\lambda_i+1)} \leq \frac{\lambda_i}{\gamma_i} = \hat{\lambda}_i$, we can obtain} 
 & \lesssim \Theta(1)\cdot \sigma^2 \bigg(\frac{k^*}{N}+\frac{N}{\hat{\lambda}^2}\sum_{i>k^*}\hat{\lambda}_i^2\bigg)\\
& \lesssim \mathrm{RidgeVarianceBound}
\end{align*}

The last inequality is due to the assumption that we are in the generalizable region where the signal-to-noise ratio is reasonable and bounded.

Combining the result for both bias and variance, we have that 
$$ \mathrm{SGDRisk} \lesssim \mathrm{RidgeRisk}.$$

For {\bf Case II}, since $0 < \gamma \leq \gamma_i$, we can set $\eta = \frac{\gamma }{ \tr (\Hb)}$ and $k_1,k_2 = k^*$. Similarly, we divide the analysis into bias and variance.

{\bf Bias.} Again, we decompose the bias of SGD into two intervals: 1) $i \leq k^*$ and 2) $i > k^*$.

We start with the second interval. For $i > k^*$, by Lemma~\ref{lemma:double_effect}, we have that,
\begin{align}
        \mathrm{SGDBiasBound}[i:\infty] & = \|\tilde{\wb}^*\big\|_{\tilde{\Hb}_{k^*:\infty}}^2 \\
        & = \|\wb^*\big\|_{\Hb_{k^*:\infty}}^2 \\
\end{align}
\begin{align}
        \mathrm{RidgeBiasBound}[i:\infty] & = \|\hat{\wb}^*\big\|_{\hat{\Hb}_{k^*:\infty}}^2 \\
        & = \|\wb^*\big\|_{\Hb_{k^*:\infty}}^2 \\
\end{align}
This leads to $$ \mathrm{RidgeBiasBound}[i:\infty]  = \mathrm{SGDBiasBound}[i:\infty].$$

For $i \leq k^*$, note that we can decompose each term of bias bound as follows,
\begin{align}
    \mathrm{SGDBiasBound[i]} &= (\tilde{\wb}^*[i])^2\frac{1}{N^2 \eta ^2\tilde{\lambda}_i}\exp \bigg(-2\eta N\tilde{\lambda}_i\bigg) \notag  \\
     &= (\wb^*[i])^2 \gamma_i \frac{1}{N^2}\frac{1}{\lambda_i/\gamma_i} \bigg (\frac{\beta\lambda_i + 1}{\eta} \bigg )^2\exp \bigg(-2\eta N\tilde{\lambda}_i\bigg) \notag \\
     &= (\hat{\wb}^*[i])^2\frac{1}{N^2}\frac{1}{\hat{\lambda_i}} \hat{\lambda}^2 \frac{1}{\hat{\lambda}^2} \bigg (\frac{\beta\lambda_i + 1}{\eta} \bigg )^2\exp \bigg(-2\eta N\tilde{\lambda}_i\bigg)  \notag\\
     &= \mathrm{RidgeBiasBound}[i]  \bigg (\frac{\beta\lambda_i + 1}{\eta \hat{\lambda}} \exp \bigg(-\eta N\tilde{\lambda}_i\bigg)\bigg )^2  \label{eq:presgd_bias1}\\
     \shortintertext{subsitute $\eta$, $\tilde{\lambda}_i$ and $\beta$ in (\ref{eq:presgd_bias1}), we get:} 
     & =  \mathrm{RidgeBiasBound}[i] \cdot \\
     & \bigg ( \frac{\left( \lambda_i N/ (\log N \tr(\Hb) \gamma_i) + 1 \right)  \tr(\Hb) \gamma_i}{\hat{\lambda}} \exp \bigg(-\frac{1}{\tr(\Hb) \gamma_1} N \frac{\gamma_i \log N \tr(\Hb)}{N}\bigg)\bigg )^2  \\
 \shortintertext{using the fact that $\kappa(\Mb) = \Theta(1)$, we get:} 
    & \lesssim  \mathrm{RidgeBiasBound}[i]  \left( \frac{\lambda_i N   }{\log N\hat{\lambda}} + \frac{\tr(\Hb)}{\hat{\lambda}}\right) \frac{1}{N}  \\
     & \lesssim \mathrm{RidgeBiasBound}[i]
\end{align}

% \begin{align}\label{eq:bias}
%     \mathrm{SGDBiasBound[i]} &= (\tilde{\wb}^*[i])^2\frac{1}{N^2 \eta ^2\tilde{\lambda}_i}\exp \bigg(-2\eta N\tilde{\lambda}_i\bigg)  \\
%      &= \tilde{\wb}^*[i]\frac{\tr(\tilde{\Hb})^2}{N^2\tilde{\lambda}_i}\exp \bigg(-\frac{2N\tilde{\lambda}_i}{\tr(\tilde{\Hb})}\bigg)\\
%      & \simeq  \wb^*[i]^2\frac{N^2 \lambda_i^2}{\log(N)^2 \tr(\Hb)^2} \frac{\tr(\Hb)^2}{N^2 \lambda_i} \exp \bigg(-\frac{2N}{\tr(\Hb)} \cdot \frac{\log(N) \tr(\Hb)}{N} \bigg) \\
%      & = \wb^*[i]^2 \frac{\tilde{\lambda}^2}{\lambda_i N^2} \frac{\lambda_i^2}{\log(N)^2 \tilde{\lambda}^2}   \\
%      & = \mathrm{RidgeBias}[i] \frac{\lambda_i^2}{\log(N)^2 \tilde{\lambda}^2} \\
%      & \leq \mathrm{RidgeBiasBound}[i]
% \end{align}

Therefore, combining the results of the two intervals above, we have that 
$$\mathrm{SGDBiasBound} \lesssim \mathrm{RidgeBiasBoud}$$

Next, let's consider variance.
\begin{align}
        \mathrm{SGDVarianceBound} & = (\sigma^2+\frac{\|\tilde{w}^*\|^2_{\Ib_{0:k^*}}+N\eta \|\tilde{w}^*\|^2_{\tilde{\Hb}_{k^*:\infty}} }{N\eta})\cdot\bigg(\frac{k^*}{N}+N\eta^2\sum_{i>k^*}\tilde{\lambda}_i^2\bigg)\\      
         & = (1+\frac{\|\tilde{w}^*\|^2_{\Ib_{0:k^*}}+N\eta \|\tilde{w}^*\|^2_{\tilde{\Hb}_{k^*:\infty}} }{N\eta \sigma^2})\cdot \sigma^2 \bigg(\frac{k^*}{N}+N\eta^2\sum_{i>k^*}\tilde{\lambda}_i^2\bigg)\\
    \shortintertext{subsititue in $\eta$:}
      & = (1+\frac{\|\tilde{w}^*\|^2_{\Ib_{0:k^*}}+N\eta \|\tilde{w}^*\|^2_{\tilde{\Hb}_{k^*:\infty}} }{N\eta \sigma^2})\cdot \sigma^2 \bigg(\frac{k^*}{N}+\frac{N}{\tr(\tilde{\Hb})}\sum_{i>k^*}\tilde{\lambda}_i^2\bigg)\\
        & = (1+\frac{\|\tilde{w}^*\|^2_{\Ib_{0:k^*}}+N\eta \|\tilde{w}^*\|^2_{\tilde{\Hb}_{k^*:\infty}} }{N\eta \sigma^2})\cdot \sigma^2 \bigg(\frac{k^*}{N}+\frac{N}{\tr(\tilde{\Hb})}\sum_{i>k^*}\frac{\hat{\lambda}_i^2}{(\beta \lambda_i + 1)}\bigg)\\
    \shortintertext{substitute the premise of the case, $\hat{\lambda} \leq \tr(\tilde{\Hb})$ and the fact that $\beta \lambda_i + 1 \geq 1$: }
    & \lesssim (1+\frac{\|\tilde{w}^*\|^2_{\Ib_{0:k^*}}+N\eta \|\tilde{w}^*\|^2_{\tilde{\Hb}_{k^*:\infty}} }{N\eta \sigma^2})\cdot \sigma^2 \bigg(\frac{k^*}{N}+\frac{N}{\hat{\lambda}}\sum_{i>k^*}\hat{\lambda}_i^2\bigg)\\
          & = (1+\frac{\|\tilde{w}^*\|^2_{\Ib_{0:k^*}}+N\eta \|\tilde{w}^*\|^2_{\tilde{\Hb}_{k^*:\infty}} }{N\eta \sigma^2})\cdot \mathrm{RidgeVarianceBound}\\
          & \lesssim  \mathrm{RidgeVarianceBound}
\end{align}
Therefore, we have that 
$$ \mathrm{SGDVarianceBound} \lesssim \mathrm{RidgeVarianceBound}$$

Combining all the result above, we have that there exists an $\eta$ such that 
$$ \mathrm{SGDRiskBound} \lesssim \mathrm{RidgeRiskBound}.$$

\end{proof}
