# Supplementary material for: Improving Implicit Regularization of SGD with Preconditioning for Least Square Problems
Source: arXiv:2403.08585 source file (2024-05-26)
Supplement: Supplementary file 10 [file precond_sgd_outperformance_ridge.tex]

\newpage
\section{Analysis of precondition SGD with standard ridge regression}

\begin{theorem}[learning rate tune]
Suppose 
$$\Gb[i] = \frac{\log(N) \tr(\Hb)}{N \lambda_i}, \quad \forall i \leq k^*,$$
$$\Gb[i] = \Ib, \mathrm{otherwise}.$$

Let $\wb_{\mathrm{sgd}}(N, \Gb; \gamma)$ and $\wb_{\mathrm{ridge}}(N; \lambda)$ be the solutions found by the pre-conditioned SGD and ridge regression respectively. Then under Assumption~\ref{}, for any least square problem instance such that the ridge regression solution is generalizable  and any $\lambda$, there exists a choice of stepsize $\gamma^*$ for precondiition-SGD such that
% Then for every problem instance that satisfies Assumption \ref{assump:data_distribution}, and every ridge regression solution in the generalizable regime, there exists a choice of stepsize $\gamma^*$ for SGD such that
\begin{align*}
L\big[\wb_{\mathrm{sgd}}(N, \Gb; \gamma^*)\big]-L(\wb^*)\lesssim L\big[\wb_{\mathrm{ridge}}(N;\lambda)\big] -L(\wb^*),
\end{align*}
\end{theorem}

\begin{proof}
By Theorem~\ref{theorem:precondition_ridge_fit}, the learning dynamic of SGD after preconditioning can be characterized by $\tilde{\Hb} = \Gb^{1/2}\Hb\Gb^{1/2}$. Then based on our choice of $\Gb$, we can obtain the following eigenspectrum of $\tilde{\Hb}$:
\begin{align*}
\tilde{\lambda}[i] = \begin{cases}
\frac{\log(N) \tr(\Hb)}{N} & i\le k^*;\\
\lambda_i &\mathrm{otherwise}.
\end{cases}
\end{align*}
Then recall the lower bound of the risk achieved by ridge regression with parameter $\lambda$:
\begin{equation}
    \begin{split}
        \mathrm{RidgeRisk}
\gtrsim \underbrace{\frac{\tilde{\lambda}^2}{ N^2}\cdot\big\|\wb^*\big\|_{\Hb_{0:k^*}^{-1}}^2 + \|\wb^*\big\|_{\Hb_{k^*:\infty}}^2}_{\mathrm{RidgeBiasBound}} 
 + \underbrace{\sigma^2\cdot\bigg(\frac{k^*}{N}+\frac{N}{\tilde{\lambda}^2}\sum_{i>k^*}\lambda_i^2\bigg)}_{\mathrm{RidgeVarianceBound}},
    \end{split}
\end{equation}
where $\tilde{\lambda} = \lambda + \sum_{i>k^*}\lambda_i$ and $k^* = \min \{k: \lambda_k \leq \frac{\lambda + \sum_{i>k}\lambda_i}{N}\}$. 

Then recall the upper bound of SGD risk is given by the following, where the parameter $k_1,k_2\in[d]$ can be arbitrarily chosen:
\begin{equation}
    \begin{split}
        \mathrm{SGDRisk}
&\lesssim \underbrace{\frac{1}{\eta^2 N^2}\cdot\big\|\exp(-N\eta \tilde{\Hb})\tilde{\wb}^*\big\|_{\tilde{\Hb}_{0:k_1}^{-1}}^2 + \|\tilde{\wb}^*\big\|_{\tilde{\Hb}_{k_1:\infty}}^2}_{\mathrm{SGDBiasBound}} \\
&\qquad + \underbrace{(\sigma^2+\frac{\|\tilde{\wb}^*\|^2_{\Ib_{0:k_2}}+N\eta \|\tilde{\wb}^*\|^2_{\tilde{\Hb}_{k_2:\infty}} }{N\eta})\cdot\bigg(\frac{k_2}{N}+N\eta^2\sum_{i>k_2}\tilde{\lambda}_i^2\bigg)}_{\mathrm{SGDVarianceBound}}.
    \end{split}
\end{equation}

Then, we divide the analysis into two cases: {\bf Case I:} $\tilde{\lambda} \geq \tr(\tilde{\Hb})$ and {\bf Case II:} $\tilde{\lambda} < \tr(\tilde{\Hb})$.

For {\bf Case I}, we have that $\frac{1}{\tilde{\lambda}} \leq \frac{1}{\tr(\tilde{\Hb})}$. We can set $\eta = \frac{1}{\tilde{\lambda}}$ and $k_1,k_2 = k^*$. We divide the analysis into bias and variance. For the bias, we have that,

\begin{equation}
    \begin{split}
        \mathrm{SGDBiasBound}
& \lesssim \frac{\tilde{\lambda}^2}{ N^2}\cdot\big\|\exp(-\frac{N\tilde{\Hb}}{\tilde{\lambda}^2})\tilde{\wb}^*\big\|_{\tilde{\Hb}_{0:k^*}^{-1}}^2 + \|\tilde{\wb}^*\big\|_{\tilde{\Hb}_{k^*:\infty}}^2 \\
&=  \frac{\tilde{\lambda}^2}{ N^2}\cdot\big\|\exp(-\frac{N\tilde{\Hb}}{\tilde{\lambda}})\tilde{\wb}^*\big\|_{\tilde{\Hb}_{0:k^*}^{-1}}^2 + \|{\wb}^*\big\|_{{\Hb}_{k^*:\infty}}^2 \\
& \lesssim \frac{\tilde{\lambda}^2}{ N^2}\cdot\big\|\exp(-\frac{N\tilde{\Hb}}{\tilde{\lambda}}) \big \|^2 \big \| \tilde{\wb}^*\big\|_{{\Hb}_{0:k^*}^{-1}}^2 + \|{\wb}^*\big\|_{{\Hb}_{k^*:\infty}}^2\\
& \lesssim \frac{\tilde{\lambda}^2}{ N^2}\cdot\big\|\exp(-\frac{N\tilde{\Hb}}{\tilde{\lambda}}) \big \|^2 \big \| {\wb}^*\big\|_{{\Hb}_{0:k^*}^{-1}}^2 + \|{\wb}^*\big\|_{{\Hb}_{k^*:\infty}}^2 \\
& \lesssim \frac{\tilde{\lambda}^2}{ N^2}\cdot \big \| {\wb}^*\big\|_{{\Hb}_{0:k^*}^{-1}}^2 + \|{\wb}^*\big\|_{{\Hb}_{k^*:\infty}}^2 \\
& = \mathrm{RidgeBiasBound}
    \end{split}
\end{equation}

For the variance we have, 

\begin{equation}
    \begin{split}
        \mathrm{SGDVarianceBound}
& \lesssim (\sigma^2+\frac{\|\tilde{\wb}^*\|^2_{\Ib_{0:k^*}}+N\eta \|\tilde{\wb}^*\|^2_{\tilde{\Hb}_{k^*:\infty}} }{N\eta})\cdot\bigg(\frac{k^*}{N}+N\eta^2\sum_{i>k^*}\tilde{\lambda}_i^2\bigg) \\
 &= (1+\frac{\|\tilde{\wb}^*\|^2_{\Ib_{0:k^*}}+N\eta \|\tilde{\wb}^*\|^2_{\tilde{\Hb}_{k^*:\infty}} }{N\eta \sigma^2})\cdot \sigma^2 \bigg(\frac{k^*}{N}+\frac{N}{\tilde{\lambda}^2}\sum_{i>k^*}{\lambda}_i^2\bigg)\\
&= (1+\frac{\|\tilde{\wb}^*\|^2_{\Ib_{0:k^*}}+N\eta \|\tilde{\wb}^*\|^2_{\tilde{\Hb}_{k^*:\infty}} }{N\eta \sigma^2})\cdot \mathrm{RidgeVarianceBound}\\
& \lesssim \mathrm{RidgeVarianceBound}
    \end{split}
\end{equation}

The last inequality is due to the assumption that we are in the generalizable region where the signal-to-noise ratio is reasonable and bounded.

Combining the result for both bias and variance, we have that 
$$ \mathrm{SGDRisk} \lesssim \mathrm{RidgeRisk}.$$

For {\bf Case II}, $\frac{1}{\tilde{\lambda}} > \frac{1}{\tr(\tilde{\Hb})}$.  $\frac{1}{\tilde{\lambda}}$ is no longer a feasible learning rate. In this case, we set $\eta = \frac{1}{\tilde{\lambda}}$ and $k_1,k_2 = k^*$. 

{\bf Bias.} With the setting, we can decompose the bias of SGD into two intervals: 1) $i \leq k^*$ and 2) $i > k^*$.

We start with the second interval. For $i > k^*$, we have that,
\begin{equation}
    \begin{split}
        \mathrm{SGDBiasBound}[i:\infty] & = \|\tilde{\wb}^*\big\|_{\tilde{\Hb}_{k^*:\infty}}^2 \\
        & = \|\wb^*\big\|_{\Hb_{k^*:\infty}}^2 \\
        & = \mathrm{RidgeBiasBound}[i:\infty].
    \end{split}
\end{equation}
The second last equality is given by Lemma~\ref{lemma:double_effect}.

For $i \leq k^*$, we have that,
\begin{equation}\label{eq:bias}
\begin{split}
     \mathrm{SGDBiasBound[i]} &= \tilde{\wb}^*[i]\frac{\tr(\tilde{\Hb})^2}{N^2\tilde{\lambda_i}}\exp(-\frac{2N\tilde{\lambda_i}}{\tr(\tilde{\Hb})})  \\
     &= \tilde{\wb}^*[i]\frac{\tr(\tilde{\Hb})^2}{N^2\tilde{\lambda_i}}\exp(-\frac{2N\tilde{\lambda_i}}{\tr(\tilde{\Hb})})\\
     % & \lesssim \tilde{\wb}^*[i]\frac{\tr(\Hb)^2}{N^2\lambda_i}\exp(-\frac{2N\tilde{\lambda_i}}{\tr(\Hb)})\\
     & \simeq  \wb^*[i]^2\frac{N^2 \lambda_i^2}{\log(N)^2 \tr(\Hb)^2} \frac{\tr(\Hb)^2}{N^2 \lambda_i} \exp(-\frac{2N}{\tr(\Hb)} \cdot \frac{\log(N) \tr(\Hb)}{N}) \\
     & = \wb^*[i]^2 \frac{\tilde{\lambda}^2}{\lambda_i N^2} \frac{\lambda_i^2}{\log(N)^2 \tilde{\lambda}^2}   \\
     & = \mathrm{RidgeBias}[i] \frac{\lambda_i^2}{\log(N)^2 \tilde{\lambda}^2} \\
     & \leq \mathrm{RidgeBiasBound}[i]
\end{split}
\end{equation}

Therefore, combining the results of the two intervals above, we have that 
$$\mathrm{SGDBiasBound} \lesssim \mathrm{RidgeBiasBoud}$$

Next, let's consider variance.

\begin{equation}
    \begin{split}
        \mathrm{SGDVarianceBound} & =(\sigma^2+\frac{\|\tilde{w}^*\|^2_{\Ib_{0:k^*}}+N\eta \|\tilde{w}^*\|^2_{\tilde{\Hb}_{k^*:\infty}} }{N\eta})\cdot\bigg(\frac{k^*}{N}+N\eta^2\sum_{i>k^*}\tilde{\lambda}_i^2\bigg)\\
         & = (1+\frac{\|\tilde{w}^*\|^2_{\Ib_{0:k^*}}+N\eta \|\tilde{w}^*\|^2_{\tilde{\Hb}_{k^*:\infty}} }{N\eta \sigma^2})\cdot \sigma^2 \bigg(\frac{k^*}{N}+N\eta^2\sum_{i>k^*}\tilde{\lambda}_i^2\bigg)\\
          & =(1+\frac{\|\tilde{w}^*\|^2_{\Ib_{0:k^*}}+N\eta \|\tilde{w}^*\|^2_{\tilde{\Hb}_{k^*:\infty}} }{N\eta \sigma^2})\cdot \mathrm{RidgeVarianceBound}\\
          & \leq  2 \cdot \mathrm{RidgeVarianceBound}\\
          & \lesssim  \mathrm{RidgeVarianceBound}
    \end{split}
\end{equation}
Therefore, we have that 
$$ \mathrm{SGDVarianceBound} \lesssim \mathrm{RidgeVarianceBound}$$

Combining the result for both bias and variance, we have that 
$$ \mathrm{SGDRisk} \lesssim \mathrm{RidgeRisk}$$
\end{proof}
