# Supplementary material for: Improving Implicit Regularization of SGD with Preconditioning for Least Square Problems
Source: arXiv:2403.08585 source file (2024-05-26)
Supplement: Supplementary file 12 [file preliminary_analysis.tex]

\section{Analysis of precondition SGD with standard ridge regression}
Because of the exponential term, it is easy to control the bias of SGD with a large enough $N$. The key challenge in the analysis reside in controlling the varaicne of SGD. Now that we do not have the freedom on using difference in sample samplexity, how to use the learning rate $\eta$ and the $\beta$ in the precondition matrix to control the gap of variance between SGD and ridge.

For the preliminary analysis, we consider the case $\Mb = \Ib$ and $\Gb = \Hb + \beta \Ib$. The goal is to find a $\beta$ for $\Gb$ and a learning rate $\eta$,
$$\mathrm{SGDRisk} \lesssim \mathrm{RidgeRisk}$$

$\Mb = \Ib$ reduces the precondition ridge regression back to the standard case with the following risk bound,

\begin{equation}
    \begin{split}
        \mathrm{RidgeRisk}
\gtrsim \underbrace{\frac{\hat{\lambda}^2}{ N^2}\cdot\big\|\wb^*\big\|_{\Hb_{0:k^*}^{-1}}^2 + \|\wb^*\big\|_{\Hb_{k^*:\infty}}^2}_{\mathrm{RidgeBiasBound}} 
 + \underbrace{\sigma^2\cdot\bigg(\frac{k^*}{N}+\frac{N}{\hat{\lambda}^2}\sum_{i>k^*}\lambda_i^2\bigg)}_{\mathrm{RidgeVarianceBound}}.
    \end{split}
\end{equation}

Recall that the SGD risk is given by the following, 

\begin{equation}
    \begin{split}
        \mathrm{SGDRisk}
\lesssim \underbrace{\frac{1}{\eta^2 N^2}\cdot\big\|\exp(-N\eta \tilde{\Hb})\tilde{\wb}^*\big\|_{\Hb_{0:k^*}^{-1}}^2 + \|\tilde{\wb}^*\big\|_{\Hb_{k^*:\infty}}^2}_{\mathrm{SGDBiasBound}}
+ \underbrace{(1+R^2)\sigma^2\cdot\bigg(\frac{k^*}{N}+N\eta^2\sum_{i>k^*}\tilde{\lambda}_i^2\bigg)}_{\mathrm{SGDVarianceBound}}.
    \end{split}
\end{equation}

Suppose $\frac{1}{\hat{\lambda}} \leq \frac{1}{\alpha \tr(\tilde{\Hb})}$ is a feasible learning rate. Then setting $\eta = \frac{1}{\hat{\lambda}}$, we have that,

\begin{equation}
    \begin{split}
        \mathrm{SGDBiasBound} & = \frac{1}{\eta^2 N^2}\cdot\big\|\exp(-N\eta \tilde{\Hb})\tilde{\wb}^*\big\|_{\tilde{\Hb}_{0:k^*}^{-1}}^2 + \|\tilde{\wb}^*\big\|_{\tilde{\Hb}_{k^*:\infty}}^2 \\
        &\leq \frac{\hat{\lambda}^2}{N^2} \cdot\big\|\exp(-N\eta \tilde{\Hb})\tilde{\wb}^*\big\|_{\tilde{\Hb}_{0:k^*}^{-1}}^2 + \|\wb^*\big\|_{\Hb_{k^*:\infty}}^2\\
        &\leq \frac{\hat{\lambda}^2}{N^2} \cdot\big\|\exp(-N\eta \tilde{\Hb})\big\|^2 \big\| \wb^*\big\|_{\Hb_{0:k^*}^{-1}}^2 + \|\wb^*\big\|_{\Hb_{k^*:\infty}}^2\\
        &\leq  \frac{\hat{\lambda}}{ N^2}\cdot\big\|\wb^*\big\|_{\Hb_{0:k^*}^{-1}}^2 + \|\wb^*\big\|_{\Hb_{k^*:\infty}}^2 \\ 
        &= \mathrm{RidgeBiasBound}
    \end{split}
\end{equation}

Now let's consider the variance, 

\begin{equation}
    \begin{split}
        \mathrm{SGDVarianceBound} & =(1+R^2)\sigma^2\cdot\bigg(\frac{k^*}{N}+\frac{N}{\hat{\lambda}^2}\sum_{i>k^*}\tilde{\lambda}_i^2\bigg)\\
        & =(1+R^2)\sigma^2\cdot\bigg(\frac{k^*}{N}+\frac{N}{\hat{\lambda}^2}\sum_{i>k^*}{\lambda_i}^2(\lambda_i+\beta)^2\bigg) \\ 
    \end{split}
\end{equation}

\jw{there is a subtle technicality issue here. Strictly speaking, the sum above can not be extended to infinity because it would diverge due to the non-zero $\beta$.}

So long as $\lambda_{k^*}+\beta \leq 1$, we have 

\jw{why do we need $\Hb$ in $\Gb$? Simply use $\beta \Ib$ as the precondition would works as well so far.}

\begin{equation}
    \begin{split}
        \mathrm{SGDVarianceBound} & =(1+R^2)\sigma^2\cdot\bigg(\frac{k^*}{N}+\frac{N}{\hat{\lambda}^2}\sum_{i>k^*}\tilde{\lambda}_i^2\bigg)\\
        & =(1+R^2)\sigma^2\cdot\bigg(\frac{k^*}{N}+\frac{N}{\hat{\lambda}^2}\sum_{i>k^*}{\lambda_i}^2(\lambda_i+\beta)^2\bigg) \\ 
        & \leq (1+R^2)\sigma^2\cdot\bigg(\frac{k^*}{N}+\frac{N}{\hat{\lambda}^2}\sum_{i>k^*}{\lambda_i}^2\bigg) \\ 
        & =  (1+R^2) \mathrm{RidgeBiasBound}
    \end{split}
\end{equation}

Therefore, we have $$\mathrm{SGDVarianceBound} \lesssim \mathrm{RidgeBiasBound}.$$

\jw{One easy route from here is to tune $\Gb$ so that it always holds $\frac{1}{\hat{\lambda}} \leq \frac{1}{\alpha \tr(\tilde{\Hb})}$}

\jw{Is the $\alpha$ factor a typo in the note? I am not sure where $\alpha$ in Theorem~\ref{theorem:precondition_sgd_fit} comes from.  What does $\alpha$ depends on, what the ranges is or what are the constraint. }

\jw{The following analysis is still loose at the moment}
Suppose $\hat{\lambda} > \alpha \tr(\tilde{\Hb})$, we set the learning rate to be largest possible $\eta = \frac{1}{\alpha \tr(\tilde{\Hb})}$,

\begin{equation}
    \begin{split}
        \mathrm{SGDBiasBound}  &\le \frac{(1-\eta\lambda_{k^*})^{2N}}{\eta^2N^2}\cdot \|\tilde{\wb}^*\|_{\tilde{\Hb}_{0:k^*}}^2 + \|\tilde{\wb}^*\|_{\tilde{\Hb}_{k^*:\infty}}^2\notag\\
    \end{split}
\end{equation}

Because $1-\eta\lambda_{k^*} < 1$, we have 
\begin{equation}
    \begin{split}
     \frac{(1-\eta\lambda_{k^*})^{2N}}{{\eta^2N^2}} /\frac{\hat{\lambda}^2}{ N^2}  \\
     = \frac{(1-\eta\lambda_{k^*})^{2N}}{\hat{\lambda}^2 \eta^2} \\
    \end{split}
\end{equation}
$$\frac{(1-\eta\lambda_{k^*})^{2N}}{\hat{\lambda}^2 \eta^2} 
     \mapsto 0,  N \mapsto \infty$$

Therefore, for a large enough $N$, we have 
\begin{equation}
    \begin{split}
        \mathrm{SGDBiasBound}  &\le \frac{(1-\eta\lambda_{k^*})^{2N}}{\eta^2N^2}\cdot \|\tilde{\wb}^*\|_{\tilde{\Hb}_{0:k^*}}^2 + \|\tilde{\wb}^*\|_{\tilde{\Hb}_{k^*:\infty}}^2\notag\\
         &\leq  \frac{\hat{\lambda}}{ N^2}\cdot\big\|\wb^*\big\|_{\Hb_{0:k^*}^{-1}}^2 + \|\wb^*\big\|_{\Hb_{k^*:\infty}}^2 \\ 
        &= \mathrm{RidgeBiasBound}
    \end{split}
\end{equation}

Now, we continue to show the variance,

\begin{equation}
    \begin{split}
        \mathrm{SGDVarianceBound} & =(1+R^2)\sigma^2\cdot\bigg(\frac{k^*}{N}+\frac{N}{\eta^2}\sum_{i>k^*}\tilde{\lambda}_i^2\bigg) \\
        & =(1+R^2)\sigma^2\cdot\bigg(\frac{k^*}{N}+\frac{N}{\eta^2}\sum_{i>k^*}{\lambda}_i^2 (\lambda_i + \beta)^2\bigg) \\
        & \leq (1+R^2)\sigma^2\cdot\bigg(\frac{k^*}{N}+\frac{N (\lambda_{k^*} + \beta)^2}{\eta^2}\sum_{i>k^*}{\lambda}_i^2 \bigg) 
    \end{split}
\end{equation}

Therefore, so long as we have 
$$\frac{ (\lambda_{k^*} + \beta)^2}{\eta^2} \leq \frac{1}{\hat{\lambda}^2}$$
We get that

\begin{equation}
    \begin{split}
        \mathrm{SGDVarianceBound} 
        & \leq (1+R^2)\sigma^2\cdot\bigg(\frac{k^*}{N}+\frac{N (\lambda_{k^*} + \beta)^2}{\eta^2}\sum_{i>k^*}{\lambda}_i^2 \bigg) \\
        & \leq (1+R^2)\sigma^2\cdot\bigg(\frac{k^*}{N}+\frac{N}{\hat{\lambda}^2}\sum_{i>k^*}{\lambda}_i^2 \bigg)\\
        & = (1+R^2) \mathrm{RidgeVarianceBound}
    \end{split}
\end{equation}

\jw{previously, we said that $\Gb = \Hb + \beta \Ib$ is a good choice but the current analysis does not suggest this is the case. Therefore, I am a bit worried I am heading at the wrong direction.}

\jw{As for the next step, I am a bit confused by the motivation of precondition ridge regression. What is the motivation for preconditioned ridge regression? what is its desired properties?}
