# Supplementary material for: Improving Implicit Regularization of SGD with Preconditioning for Least Square Problems
Source: arXiv:2403.08585 source file (2024-05-26)
Supplement: Supplementary file 13 [file preliminary_analysis2_inverse.tex]

\section{Analysis of precondition SGD with standard ridge regression}
\jw{add beta only on the portion of eigenvector that are not too large or too small}

Because of the exponential term, it is easy to control the bias of SGD with a large enough $N$. The key challenge in the analysis resides in controlling the varaicne of SGD. Now that we do not have the freedom on using difference in sample samplexity, how to use the learning rate $\eta$ and the $\beta$ in the precondition matrix to control the gap of variance between SGD and ridge.

For the preliminary analysis, we consider the case $\Mb = \Ib$ and $\Gb = (\Hb + \beta \Ib)^{-1}$. The goal is to find a $\beta$ for $\Gb$ and a learning rate $\eta$,
$$\mathrm{SGDRisk} \lesssim \mathrm{RidgeRisk}$$

$\Mb = \Ib$ reduces the precondition ridge regression back to the standard case with the following risk bound,

\begin{equation}
    \begin{split}
        \mathrm{RidgeRisk}
\gtrsim \underbrace{\frac{\hat{\lambda}^2}{ N^2}\cdot\big\|\wb^*\big\|_{\Hb_{0:k^*}^{-1}}^2 + \|\wb^*\big\|_{\Hb_{k^*:\infty}}^2}_{\mathrm{RidgeBiasBound}} 
 + \underbrace{\sigma^2\cdot\bigg(\frac{k^*}{N}+\frac{N}{\hat{\lambda}^2}\sum_{i>k^*}\lambda_i^2\bigg)}_{\mathrm{RidgeVarianceBound}}.
    \end{split}
\end{equation}

Recall that the SGD risk is given by the following, 

\begin{equation}
    \begin{split}
        \mathrm{SGDRisk}
\lesssim \underbrace{\frac{1}{\eta^2 N^2}\cdot\big\|\exp(-N\eta \tilde{\Hb})\tilde{\wb}^*\big\|_{\Hb_{0:k^*}^{-1}}^2 + \|\tilde{\wb}^*\big\|_{\Hb_{k^*:\infty}}^2}_{\mathrm{SGDBiasBound}}
+ \underbrace{(1+R^2)\sigma^2\cdot\bigg(\frac{k^*}{N}+N\eta^2\sum_{i>k^*}\tilde{\lambda}_i^2\bigg)}_{\mathrm{SGDVarianceBound}}.
    \end{split}
\end{equation}

Suppose $\frac{1}{\hat{\lambda}} \leq \frac{1}{\alpha \tr(\tilde{\Hb})}$ is a feasible learning rate. Then setting $\eta = \frac{1}{\hat{\lambda}}$, we have that,

\begin{equation}
    \begin{split}
        \mathrm{SGDBiasBound} & = \frac{1}{\eta^2 N^2}\cdot\big\|\exp(-N\eta \tilde{\Hb})\tilde{\wb}^*\big\|_{\tilde{\Hb}_{0:k^*}^{-1}}^2 + \|\tilde{\wb}^*\big\|_{\tilde{\Hb}_{k^*:\infty}}^2 \\
        &\leq \frac{\hat{\lambda}^2}{N^2} \cdot\big\|\exp(-N\eta \tilde{\Hb})\tilde{\wb}^*\big\|_{\tilde{\Hb}_{0:k^*}^{-1}}^2 + \|\wb^*\big\|_{\Hb_{k^*:\infty}}^2\\
        &\leq \frac{\hat{\lambda}^2}{N^2} \cdot\big\|\exp(-N\eta \tilde{\Hb})\big\|^2 \big\| \wb^*\big\|_{\Hb_{0:k^*}^{-1}}^2 + \|\wb^*\big\|_{\Hb_{k^*:\infty}}^2\\
        &\leq  \frac{\hat{\lambda}^2}{ N^2}\cdot\big\|\wb^*\big\|_{\Hb_{0:k^*}^{-1}}^2 + \|\wb^*\big\|_{\Hb_{k^*:\infty}}^2 \\ 
        &= \mathrm{RidgeBiasBound}
    \end{split}
\end{equation}

Now let's consider the variance, 

\begin{equation}
    \begin{split}
        \mathrm{SGDVarianceBound} & =(1+R^2)\sigma^2\cdot\bigg(\frac{k^*}{N}+\frac{N}{\hat{\lambda}^2}\sum_{i>k^*}\tilde{\lambda}_i^2\bigg)\\
        & =(1+R^2)\sigma^2\cdot\bigg(\frac{k^*}{N}+\frac{N}{\hat{\lambda}^2}\sum_{i>k^*}\frac{{\lambda_i}^2}{(\lambda_i+\beta)^2}\bigg) \\ 
    \end{split}
\end{equation}

So long as $\lambda_i+\beta \geq 1$, we have

\begin{equation}
    \begin{split}
        \mathrm{SGDVarianceBound} & =(1+R^2)\sigma^2\cdot\bigg(\frac{k^*}{N}+\frac{N}{\hat{\lambda}^2}\sum_{i>k^*}\tilde{\lambda}_i^2\bigg)\\
        & =(1+R^2)\sigma^2\cdot\bigg(\frac{k^*}{N}+\frac{N}{\hat{\lambda}^2}\sum_{i>k^*}\frac{{\lambda_i}^2}{(\lambda_i+\beta)^2}\bigg) \\ 
        & \leq (1+R^2)\sigma^2\cdot\bigg(\frac{k^*}{N}+\frac{N}{\hat{\lambda}^2}\sum_{i>k^*}\frac{1}{\beta^2} {\lambda_i}^2\bigg) \\ 
        & \leq (1+R^2)\sigma^2\cdot\bigg(\frac{k^*}{N}+\frac{N}{\hat{\lambda}^2}\sum_{i>k^*}{\lambda_i}^2\bigg) \\ 
        & =  (1+R^2) \mathrm{RidgeBiasBound}
    \end{split}
\end{equation}

Therefore, we have $$\mathrm{SGDVarianceBound} \lesssim \mathrm{RidgeBiasBound}.$$

\jw{One easy route from here is to tune $\Gb$ so that it always holds $\frac{1}{\hat{\lambda}} \leq \frac{1}{\alpha \tr(\tilde{\Hb})}$}

This leads to 
\begin{equation}
    \begin{split}
        \frac{1}{\hat{\lambda}} & \leq \frac{1}{\alpha \tr(\tilde{\Hb})}\\
        \alpha \tr(\tilde{\Hb}) & \leq \hat{\lambda} \\
        \alpha \sum \frac{\lambda_i}{\lambda_i + \beta} &\leq \hat{\lambda} \\
        \beta &\geq \sum (\frac{\alpha}{\hat{\lambda}} - 1)\lambda_i
    \end{split}
\end{equation}

\jw{The following analysis is still loose at the moment}

Suppose $\hat{\lambda} > \alpha \tr(\tilde{\Hb})$, we set the learning rate to be largest possible $\eta = \frac{1}{\alpha \tr(\tilde{\Hb})}$,

\begin{equation}
    \begin{split}
        \mathrm{SGDBiasBound}  &\le \frac{(1-\eta\lambda_{k^*})^{2N}}{\eta^2N^2}\cdot \|\tilde{\wb}^*\|_{\tilde{\Hb}_{0:k^*}}^2 + \|\tilde{\wb}^*\|_{\tilde{\Hb}_{k^*:\infty}}^2\notag\\
    \end{split}
\end{equation}

Because $1-\eta\lambda_{k^*} < 1$, we have 
\begin{equation}
    \begin{split}
     \frac{(1-\eta\lambda_{k^*})^{2N}}{{\eta^2N^2}} /\frac{\hat{\lambda}^2}{ N^2}  \\
     = \frac{(1-\eta\lambda_{k^*})^{2N}}{\hat{\lambda}^2 \eta^2} \\
    \end{split}
\end{equation}
$$\frac{(1-\eta\lambda_{k^*})^{2N}}{\hat{\lambda}^2 \eta^2} 
     \mapsto 0,  N \mapsto \infty$$

Therefore, for a large enough $N$, we have 
\begin{equation}
    \begin{split}
        \mathrm{SGDBiasBound}  &\le \frac{(1-\eta\lambda_{k^*})^{2N}}{\eta^2N^2}\cdot \|\tilde{\wb}^*\|_{\tilde{\Hb}_{0:k^*}}^2 + \|\tilde{\wb}^*\|_{\tilde{\Hb}_{k^*:\infty}}^2\notag\\
         &\leq  \frac{\hat{\lambda}}{ N^2}\cdot\big\|\wb^*\big\|_{\Hb_{0:k^*}^{-1}}^2 + \|\wb^*\big\|_{\Hb_{k^*:\infty}}^2 \\ 
        &= \mathrm{RidgeBiasBound}
    \end{split}
\end{equation}

Now, we continue to show the variance,

\begin{equation}
    \begin{split}
        \mathrm{SGDVarianceBound} & =(1+R^2)\sigma^2\cdot\bigg(\frac{k^*}{N}+\frac{N}{\eta^2}\sum_{i>k^*}\tilde{\lambda}_i^2\bigg) \\
        & =(1+R^2)\sigma^2\cdot\bigg(\frac{k^*}{N}+\frac{N}{\eta^2}\sum_{i>k^*}\frac{{\lambda_i}^2}{(\lambda_i+\beta)^2}\bigg) \\
        & \leq (1+R^2)\sigma^2\cdot\bigg(\frac{k^*}{N}+\frac{N}{\eta^2 \beta^2}\sum_{i>k^*}{\lambda}_i^2 \bigg) 
    \end{split}
\end{equation}

Therefore, so long as we have 
% \begin{equation}
%     \begin{split}
%         \frac{N}{\eta^2 \beta^2} & \leq \frac{1}{\hat{\lambda}^2}\\
%         \beta^2 & \geq \frac{\hat{\lambda}^2N}{\eta^2}
%     \end{split}
% \end{equation}

\begin{equation}
    \begin{split}
        \frac{1}{\eta^2 (\lambda_i + \beta)^2} & \leq \frac{1}{\hat{\lambda}^2}\\
        (\lambda_i + \beta)^2 & \geq \frac{\hat{\lambda}^2}{\eta^2}
    \end{split}
\end{equation}

We get that

\begin{equation}
    \begin{split}
        \mathrm{SGDVarianceBound} 
        & \leq (1+R^2)\sigma^2\cdot\bigg(\frac{k^*}{N}+\frac{N}{\eta^2 \beta^2}\sum_{i>k^*}{\lambda}_i^2 \bigg) \\
        & \leq (1+R^2)\sigma^2\cdot\bigg(\frac{k^*}{N}+\frac{N}{\hat{\lambda}^2}\sum_{i>k^*}{\lambda}_i^2 \bigg)\\
        & = (1+R^2) \mathrm{RidgeVarianceBound}
      \end{split}
\end{equation}

\jw{Is the $\alpha$ factor a typo in the note? I am not sure where $\alpha$ in Theorem~\ref{theorem:precondition_sgd_fit} comes from.  What does $\alpha$ depends on, what the ranges is or what are the constraint. }

\jw{why do we need $\Hb$ in $\Gb$? Simply use $\beta \Ib$ as the precondition would work as well so far. Not clear the role of $\Hb$ in $\Gb$}

\jw{As for the next step, I am a bit confused by the motivation of precondition ridge regression. What is the motivation for preconditioned ridge regression? what is its desired properties?}

\jw{When can we ignore some constant?}
