# Supplementary material for: Improving Implicit Regularization of SGD with Preconditioning for Least Square Problems
Source: arXiv:2403.08585 source file (2024-05-26)
Supplement: Supplementary file 14 [file preliminary_analysis_with_conditioned_ridge.tex]

\section{Analysis of precondition SGD with conditioned ridge regression}

For this analysis, we consider the case $\Mb = \Hb + \lambda \Ib$ and $\Gb = (\Hb + \beta \Ib)^{-1}$. The choice of $\Mb$ is from the paper~\citep{gonen2016solving} which is based on the result that $\Mb = \Hb + \lambda \Ib$ yields the optimal average condition number.

The goal is to find a $\beta$ for $\Gb$ and a learning rate $\eta$,
$$\mathrm{SGDRisk} \lesssim \mathrm{RidgeRisk}$$

Based on Theorem~\ref{theorem:precondition_ridge_fit}, we have,
\begin{equation}
    \begin{split}
        \mathrm{RidgeRisk}
\gtrsim \underbrace{\frac{\hat{\lambda}}{ N^2}\cdot\big\|\hat{\wb}^*\big\|_{\hat{\Hb}_{0:k^*}^{-1}}^2 + \|\hat{\wb}^*\big\|_{\hat{\Hb}_{k^*:\infty}}^2}_{\mathrm{RidgeBiasBound}} 
 + \underbrace{\sigma^2\cdot\bigg(\frac{k^*}{N}+\frac{N}{\hat{\lambda}^2}\sum_{i>k^*}\hat{\lambda}_i^2\bigg)}_{\mathrm{RidgeVarianceBound}}.
    \end{split}
\end{equation}

Recall that the SGD risk is given by the following, 

\begin{equation}
    \begin{split}
        \mathrm{SGDRisk}
\lesssim \underbrace{\frac{1}{\eta^2 N^2}\cdot\big\|\exp(-N\eta \tilde{\Hb})\tilde{\wb}^*\big\|_{\Hb_{0:k^*}^{-1}}^2 + \|\tilde{\wb}^*\big\|_{\Hb_{k^*:\infty}}^2}_{\mathrm{SGDBiasBound}}
+ \underbrace{(1+R^2)\sigma^2\cdot\bigg(\frac{k^*}{N}+N\eta^2\sum_{i>k^*}\tilde{\lambda}_i^2\bigg)}_{\mathrm{SGDVarianceBound}}.
    \end{split}
\end{equation}

Suppose $\frac{1}{\hat{\lambda}} \leq \frac{1}{\alpha \tr(\tilde{\Hb})}$ is a feasible learning rate. Then setting $\eta = \frac{1}{\hat{\lambda}}$, we have that,

\begin{equation}
    \begin{split}
        \mathrm{SGDBiasBound} & = \frac{1}{\eta^2 N^2}\cdot\big\|\exp(-N\eta \tilde{\Hb})\tilde{\wb}^*\big\|_{\tilde{\Hb}_{0:k^*}^{-1}}^2 + \|\tilde{\wb}^*\big\|_{\tilde{\Hb}_{k^*:\infty}}^2 \\
        &\leq \frac{\hat{\lambda}^2}{N^2} \cdot\big\|\exp(-N\eta \tilde{\Hb})\tilde{\wb}^*\big\|_{\tilde{\Hb}_{0:k^*}^{-1}}^2 + \|\wb^*\big\|_{\Hb_{k^*:\infty}}^2\\
        &\leq \frac{\hat{\lambda}^2}{N^2} \cdot\big\|\exp(-N\eta \tilde{\Hb})\big\|^2 \big\| \wb^*\big\|_{\Hb_{0:k^*}^{-1}}^2 + \|\wb^*\big\|_{\Hb_{k^*:\infty}}^2\\
        &\leq  \frac{\hat{\lambda}^2}{ N^2}\cdot\big\|\wb^*\big\|_{\Hb_{0:k^*}^{-1}}^2 + \|\wb^*\big\|_{\Hb_{k^*:\infty}}^2 \\ 
        &= \mathrm{RidgeBiasBound}
    \end{split}
\end{equation}

Now let's consider the variance, 

\begin{equation}
    \begin{split}
        \mathrm{SGDVarianceBound} & =(1+R^2)\sigma^2\cdot\bigg(\frac{k^*}{N}+\frac{N}{\hat{\lambda}^2}\sum_{i>k^*}\tilde{\lambda}_i^2\bigg)\\
        & =(1+R^2)\sigma^2\cdot\bigg(\frac{k^*}{N}+\frac{N}{\hat{\lambda}^2}\sum_{i>k^*}\frac{{\lambda_i}^2}{(\lambda_i+\beta)^2}\bigg) \\ 
    \end{split}
\end{equation}

So long as $\lambda_i+\beta \leq \lambda_i + \lambda$, we have

\begin{equation}
    \begin{split}
        \mathrm{SGDVarianceBound} & =(1+R^2)\sigma^2\cdot\bigg(\frac{k^*}{N}+\frac{N}{\hat{\lambda}^2}\sum_{i>k^*}\tilde{\lambda}_i^2\bigg)\\
        & =(1+R^2)\sigma^2\cdot\bigg(\frac{k^*}{N}+\frac{N}{\hat{\lambda}^2}\sum_{i>k^*}\frac{{\lambda_i}^2}{(\lambda_i+\beta)^2}\bigg) \\ 
        & \leq (1+R^2)\sigma^2\cdot\bigg(\frac{k^*}{N}+\frac{N}{\hat{\lambda}^2}\sum_{i>k^*} \frac{{\lambda_i}^2}{(\lambda_i+\lambda)^2}\bigg)\\ 
        & =  (1+R^2) \mathrm{RidgeBiasBound}
    \end{split}
\end{equation}

Therefore, we have $$\mathrm{SGDVarianceBound} \lesssim \mathrm{RidgeBiasBound}.$$

\jw{One easy route from here is to tune $\Gb$ so that it always holds $\frac{1}{\hat{\lambda}} \leq \frac{1}{\alpha \tr(\tilde{\Hb})}$}

This leads to 
\begin{equation}
    \begin{split}
        \frac{1}{\hat{\lambda}} & \leq \frac{1}{\alpha \tr(\tilde{\Hb})}\\
        \alpha \tr(\tilde{\Hb}) & \leq \hat{\lambda} \\
        \alpha \sum \frac{\lambda_i}{\lambda_i + \beta} &\leq \hat{\lambda} \\
        \beta &\geq \sum (\frac{\alpha}{\hat{\lambda}} - 1)\lambda_i
    \end{split}
\end{equation}

\jw{The following analysis is still loose at the moment}

Suppose $\hat{\lambda} > \alpha \tr(\tilde{\Hb})$, we set the learning rate to be largest possible $\eta = \frac{1}{\alpha \tr(\tilde{\Hb})}$,

\begin{equation}
    \begin{split}
        \mathrm{SGDBiasBound}  &\le \frac{(1-\eta\lambda_{k^*})^{2N}}{\eta^2N^2}\cdot \|\tilde{\wb}^*\|_{\tilde{\Hb}_{0:k^*}}^2 + \|\tilde{\wb}^*\|_{\tilde{\Hb}_{k^*:\infty}}^2\notag\\
    \end{split}
\end{equation}

Because $1-\eta\lambda_{k^*} < 1$, we have 
\begin{equation}
    \begin{split}
     \frac{(1-\eta\lambda_{k^*})^{2N}}{{\eta^2N^2}} /\frac{\hat{\lambda}^2}{ N^2}  \\
     = \frac{(1-\eta\lambda_{k^*})^{2N}}{\hat{\lambda}^2 \eta^2} \\
    \end{split}
\end{equation}
$$\frac{(1-\eta\lambda_{k^*})^{2N}}{\hat{\lambda}^2 \eta^2} 
     \mapsto 0,  N \mapsto \infty$$

Therefore, for a large enough $N$, we have 
\begin{equation}
    \begin{split}
        \mathrm{SGDBiasBound}  &\le \frac{(1-\eta\lambda_{k^*})^{2N}}{\eta^2N^2}\cdot \|\tilde{\wb}^*\|_{\tilde{\Hb}_{0:k^*}}^2 + \|\tilde{\wb}^*\|_{\tilde{\Hb}_{k^*:\infty}}^2\notag\\
         &\leq  \frac{\hat{\lambda}}{ N^2}\cdot\big\|\wb^*\big\|_{\Hb_{0:k^*}^{-1}}^2 + \|\wb^*\big\|_{\Hb_{k^*:\infty}}^2 \\ 
         &=  \frac{\hat{\lambda}}{ N^2}\cdot\big\|\hat{\wb}^*\big\|_{\hat{\Hb}_{0:k^*}^{-1}}^2 + \|\hat{\wb}^*\big\|_{\hat{\Hb}_{k^*:\infty}}^2 \\ 
        &= \mathrm{RidgeBiasBound}
    \end{split}
\end{equation}

Now, we continue to show the variance,

\begin{equation}
    \begin{split}
        \mathrm{SGDVarianceBound} & =(1+R^2)\sigma^2\cdot\bigg(\frac{k^*}{N}+\frac{N}{\eta^2}\sum_{i>k^*}\tilde{\lambda}_i^2\bigg) \\
        & =(1+R^2)\sigma^2\cdot\bigg(\frac{k^*}{N}+\frac{N}{\eta^2}\sum_{i>k^*}\frac{{\lambda_i}^2}{(\lambda_i+\beta)^2}\bigg) \\
        & \leq (1+R^2)\sigma^2\cdot\bigg(\frac{k^*}{N}+\frac{N}{\eta^2 \beta^2}\sum_{i>k^*}{\lambda}_i^2 \bigg) 
    \end{split}
\end{equation}

Therefore, so long as we have 
% \begin{equation}
%     \begin{split}
%         \frac{N}{\eta^2 \beta^2} & \leq \frac{1}{\hat{\lambda}^2}\\
%         \beta^2 & \geq \frac{\hat{\lambda}^2N}{\eta^2}
%     \end{split}
% \end{equation}

\begin{equation}
    \begin{split}
        \frac{1}{\eta^2 (\lambda_i + \beta)^2} & \leq \frac{1}{\hat{\lambda}^2 (\lambda_i + \lambda)^2}\\
        \frac{(\lambda_i + \lambda)^2}{(\lambda_i + \beta)^2} & \geq \frac{\hat{\lambda}^2}{\eta^2}
    \end{split}
\end{equation}

We get that

\begin{equation}
    \begin{split}
        \mathrm{SGDVarianceBound} 
        & \leq (1+R^2)\sigma^2\cdot\bigg(\frac{k^*}{N}+\frac{N}{\eta^2}\sum_{i>k^*}\frac{{\lambda_i}^2}{(\lambda_i+\beta)^2}\bigg) \\
        & \leq (1+R^2)\sigma^2\cdot\bigg(\frac{k^*}{N}+\frac{N}{\eta^2}\sum_{i>k^*}\frac{{\lambda_i}^2}{(\lambda_i+\lambda)^2}\bigg) \\
        & = (1+R^2) \mathrm{RidgeVarianceBound}
      \end{split}
\end{equation}
